# Supplementary material for: An inferential measure of dependence between two systems using Bayesian model comparison
Source: arXiv:2412.06478 ancillary file (2024-12-10)
Supplement: Supplementary file 1 [file Supplement.pdf]

# Supplementary material for manuscript “An inferential measure of dependence between two systems using Bayesian model comparison”

Guillaume Marrelec and Alain Giron

## Contents

|           |                                                              |           |
|-----------|--------------------------------------------------------------|-----------|
| <b>1</b>  | <b>Known distributions</b>                                   | <b>3</b>  |
| 1.1       | Case of independence . . . . .                               | 3         |
| 1.2       | Case of dependence . . . . .                                 | 4         |
| <b>2</b>  | <b>Known likelihood functions with unknown parameters</b>    | <b>4</b>  |
| <b>3</b>  | <b>Nested models</b>                                         | <b>5</b>  |
| <b>4</b>  | <b>Maximum-entropy distributions</b>                         | <b>6</b>  |
| 4.1       | Summary of results . . . . .                                 | 6         |
| 4.2       | Intermediary results . . . . .                               | 6         |
| <b>5</b>  | <b>Multivariate normal distributions</b>                     | <b>8</b>  |
| 5.1       | Summary of results . . . . .                                 | 8         |
| 5.2       | Intermediary results . . . . .                               | 9         |
| <b>6</b>  | <b>Bivariate discrete distributions</b>                      | <b>11</b> |
| 6.1       | Summary of results . . . . .                                 | 11        |
| 6.2       | Intermediary results . . . . .                               | 12        |
| <b>7</b>  | <b>Model misspecification</b>                                | <b>14</b> |
| 7.1       | Known distributions . . . . .                                | 14        |
| 7.2       | Known likelihood functions with unknown parameters . . . . . | 15        |
| <b>8</b>  | <b>Bivariate normal distribution with noise</b>              | <b>15</b> |
| 8.1       | Graphical model . . . . .                                    | 15        |
| 8.2       | Marginal model likelihood of $H_0$ . . . . .                 | 15        |
| 8.3       | Marginal model likelihood of $H_1$ . . . . .                 | 17        |
| <b>9</b>  | <b>Functional dependence plus noise</b>                      | <b>18</b> |
| 9.1       | Graphical model . . . . .                                    | 18        |
| 9.2       | Marginal model likelihood of $H_0$ . . . . .                 | 18        |
| 9.3       | Marginal model likelihood of $H_1$ . . . . .                 | 20        |
| <b>10</b> | <b>Phase synchronization of chaotic systems</b>              | <b>21</b> |
| <b>11</b> | <b>Real-life application</b>                                 | <b>21</b> |
| 11.1      | Case of independence . . . . .                               | 21        |
| 11.2      | Case of dependence . . . . .                                 | 22        |
| 11.3      | Measure of dependence . . . . .                              | 22        |

|                                                       |           |
|-------------------------------------------------------|-----------|
| <b>12 The case of the log Bayes ratio per sample</b>  | <b>22</b> |
| 12.1 Definition . . . . .                             | 22        |
| 12.2 Calculations . . . . .                           | 22        |
| 12.3 Simulation studies . . . . .                     | 23        |
| 12.4 Summary . . . . .                                | 25        |
| <b>13 Mutual information for the simulation study</b> | <b>25</b> |

# 1 Known distributions

We assume that the distribution of  $(X, Y)$  is known exactly in both  $H_0$  and  $H_1$ . In this case, we remove the explicit dependency on the model parameter for the sake of simplicity. Equation (10) of the manuscript leads to

$$\begin{aligned}\mathfrak{B}_{\text{lnr}}(\mathcal{X}, \mathcal{Y}|D) &= \ln \frac{p(H_1)}{p(H_0)} + \ln \frac{\prod_{n=1}^N f_{XY}^{(1)}(\mathbf{x}_n, \mathbf{y}_n)}{\prod_{n=1}^N f_X^{(0)}(\mathbf{x}_n) f_Y^{(0)}(\mathbf{y}_n)} \\ &= \ln \frac{p(H_1)}{p(H_0)} + \sum_{n=1}^N \ln \frac{f_{XY}^{(1)}(\mathbf{x}_n, \mathbf{y}_n)}{f_X^{(0)}(\mathbf{x}_n) f_Y^{(0)}(\mathbf{y}_n)}.\end{aligned}\quad (\text{S-1})$$

Setting

$$J_N(D) = \frac{1}{N} \sum_{n=1}^N \ln \frac{f_{XY}^{(1)}(\mathbf{x}_n, \mathbf{y}_n)}{f_X^{(0)}(\mathbf{x}_n) f_Y^{(0)}(\mathbf{y}_n)}, \quad (\text{S-2})$$

we obtain

$$\mathfrak{B}_{\text{lnr}}(\mathcal{X}, \mathcal{Y}|D) = \ln \frac{p(H_1)}{p(H_0)} + N J_N(D). \quad (\text{S-3})$$

According to the strong law of large numbers (Bernardo and Smith, 2000, §3.2.3),  $J_N(D)$  tends to

$$\int f(\mathbf{x}, \mathbf{y}) \ln \frac{f_{XY}^{(1)}(\mathbf{x}, \mathbf{y})}{f_X^{(0)}(\mathbf{x}) f_Y^{(0)}(\mathbf{y})} d\mathbf{x} d\mathbf{y} \quad (\text{S-4})$$

when  $N \rightarrow \infty$ , where  $f(\mathbf{x}, \mathbf{y})$  is the true underlying distribution of  $(X, Y)$ . We can now consider what happens under the assumptions of independence (§1.1) and dependence (§1.2).

## 1.1 Case of independence

If  $H_0$  is true,  $f(\mathbf{x}, \mathbf{y})$  is equal to  $f_X^{(0)}(\mathbf{x}) f_Y^{(0)}(\mathbf{y})$ . The expression of Equation (S-4) is then equal to  $-D_{\text{KL}}(f_X^{(0)} f_Y^{(0)} \| f_{XY}^{(1)})$ , where  $D_{\text{KL}}(u \| v)$  is the relative entropy (or Kullback–Leibler divergence) between  $u(\mathbf{z})$  and  $v(\mathbf{z})$ ,

$$D_{\text{KL}}(u \| v) = \int u(\mathbf{z}) \ln \frac{u(\mathbf{z})}{v(\mathbf{z})} d\mathbf{z}.$$

Since the Kullback–Leibler divergence between two distinct distributions is always strictly positive, we have

$$J_N(D) \xrightarrow{N \rightarrow \infty} -D_{\text{KL}}(f_X^{(0)} f_Y^{(0)} \| f_{XY}^{(1)}) < 0.$$

$J_N(D)$  will therefore be strictly negative for  $N$  large enough. As a consequence,  $\mathfrak{B}_{\text{lnr}}(\mathcal{X}, \mathcal{Y}|D)$  of Equation (S-3) will tend to  $-\infty$  as  $N \rightarrow \infty$ .

Besides, the sampling expectation of  $\mathfrak{B}_{\text{lnr}}(\mathcal{X}, \mathcal{Y}|D)$  under  $H_0$  for finite  $N$  can be obtained from Equation (S-1) as

$$\begin{aligned}\mathbb{E}[\mathfrak{B}_{\text{lnr}}(\mathcal{X}, \mathcal{Y}|D)|H_0] &= \ln \frac{p(H_1)}{p(H_0)} + N \int f_X^{(0)}(\mathbf{x}) f_Y^{(0)}(\mathbf{y}) \ln \frac{f_{XY}^{(1)}(\mathbf{x}, \mathbf{y})}{f_X^{(0)}(\mathbf{x}) f_Y^{(0)}(\mathbf{y})} d\mathbf{x} d\mathbf{y} \\ &= \ln \frac{p(H_1)}{p(H_0)} - N D_{\text{KL}}(f_X^{(0)} f_Y^{(0)} \| f_{XY}^{(1)}).\end{aligned}$$

This is a decreasing function of  $D_{\text{KL}}(f_X^{(0)} f_Y^{(0)} \| f_{XY}^{(1)})$ . Since  $D_{\text{KL}}(f_X^{(0)} f_Y^{(0)} \| f_{XY}^{(1)}) > 0$ , it is also a decreasing function of  $N$ .

## 1.2 Case of dependence

By contrast, if  $H_1$  is true,  $f(\mathbf{x}, \mathbf{y})$  of Equation (S-4) is equal to  $f_{XY}^{(1)}(\mathbf{x}, \mathbf{y})$ . As  $N \rightarrow \infty$ ,  $J_N(D)$  tends to  $D_{\text{KL}}(f_{XY}^{(1)} \| f_X^{(0)} f_Y^{(0)})$ , i.e.,

$$\int f_{XY}^{(1)}(\mathbf{x}, \mathbf{y}) \ln \frac{f_{XY}^{(1)}(\mathbf{x}, \mathbf{y})}{f_X^{(0)}(\mathbf{x}) f_Y^{(0)}(\mathbf{y})} d\mathbf{x} d\mathbf{y}.$$

This can be reexpressed as

$$\int f_{XY}^{(1)}(\mathbf{x}, \mathbf{y}) \ln \frac{f_{XY}^{(1)}(\mathbf{x}, \mathbf{y})}{f_X^{(1)}(\mathbf{x}) f_Y^{(1)}(\mathbf{y})} d\mathbf{x} d\mathbf{y} + \int f_{XY}^{(1)}(\mathbf{x}, \mathbf{y}) \ln \frac{f_X^{(1)}(\mathbf{x}) f_Y^{(1)}(\mathbf{y})}{f_X^{(0)}(\mathbf{x}) f_Y^{(0)}(\mathbf{y})} d\mathbf{x} d\mathbf{y},$$

where  $f_X^{(1)}(\mathbf{x})$  and  $f_Y^{(1)}(\mathbf{y})$  are the marginals of  $X$  and  $Y$ , respectively, under  $H_1$ . The first integral is equal to  $D_{\text{KL}}(f_{XY}^{(1)} \| f_X^{(1)} f_Y^{(1)})$ , also called mutual information between  $X$  and  $Y$  (Cover and Thomas, 1991, Chap. 2) and denoted by  $I(X, Y)$ . The second integral is equal to  $D_{\text{KL}}(f_X^{(1)} \| f_X^{(0)}) + D_{\text{KL}}(f_Y^{(1)} \| f_Y^{(0)})$ . Since  $I(X, Y)$  is strictly positive under  $H_1$  and both  $D_{\text{KL}}(f_X^{(1)} \| f_X^{(0)})$  and  $D_{\text{KL}}(f_Y^{(1)} \| f_Y^{(0)})$  are positive as Kullback–Leibler divergences, we have that  $J_N(D)$  tends to

$$I(X, Y) + D_{\text{KL}}(f_X^{(1)} \| f_X^{(0)}) + D_{\text{KL}}(f_Y^{(1)} \| f_Y^{(0)}) > 0$$

as  $N \rightarrow \infty$ .  $J_N(D)$  will therefore be strictly positive for  $N$  large enough. Consequently,  $\mathfrak{B}_{\text{lnr}}(\mathcal{X}, \mathcal{Y} | D)$  will tend to  $+\infty$  as  $N \rightarrow \infty$ .

Besides, if  $H_1$  is true, then the sampling expectation of  $\mathfrak{B}_{\text{lnr}}(\mathcal{X}, \mathcal{Y} | D)$  for finite  $N$  is given by

$$\begin{aligned} \mathbb{E}[\mathfrak{B}_{\text{lnr}}(\mathcal{X}, \mathcal{Y} | D) | H_1] &= \ln \frac{p(H_1)}{p(H_0)} + N \int f_{XY}^{(1)}(\mathbf{x}, \mathbf{y}) \ln \frac{f_{XY}^{(1)}(\mathbf{x}, \mathbf{y})}{f_X^{(0)}(\mathbf{x}) f_Y^{(0)}(\mathbf{y})} d\mathbf{x} d\mathbf{y} \\ &= \ln \frac{p(H_1)}{p(H_0)} + N \left[ I(X, Y) + D_{\text{KL}}(f_X^{(1)} \| f_X^{(0)}) + D_{\text{KL}}(f_Y^{(1)} \| f_Y^{(0)}) \right]. \end{aligned}$$

This is an increasing function of  $I(X, Y)$ . Since  $I(X, Y)$  is always strictly positive under  $H_1$  and both  $D_{\text{KL}}(f_X^{(1)} \| f_X^{(0)})$  and  $D_{\text{KL}}(f_Y^{(1)} \| f_Y^{(0)})$  are positive, the expectation is also an increasing function of  $N$ .

## 2 Known likelihood functions with unknown parameters

Assuming that the prior  $h_i(\boldsymbol{\theta}^{(i)})$  is strictly positive and of slow variation around  $\hat{\boldsymbol{\theta}}_N^{(i)}$ , the integral of Equation (11) of the manuscript can be approximated using Laplace method (Tierney and Kadane, 1986; Gelfand and Dey, 1994), yielding

$$P(D | H_i) = \frac{h_i(\hat{\boldsymbol{\theta}}_N^{(i)}) L_i(\hat{\boldsymbol{\theta}}_N^{(i)}) (2\pi)^{\frac{D_i}{2}}}{N^{\frac{D_i}{2}} \left| \sqrt{\det(\mathbf{G}^{(i)})} \right|} \left[ 1 + O\left(\frac{1}{N}\right) \right], \quad (\text{S-5})$$

where  $O(\cdot)$  stands for the usual Bachmann–Landau, Big  $O$  notation and  $\mathbf{G}^{(i)}$  is the average of sampling Hessian matrices at  $\hat{\boldsymbol{\theta}}_N^{(i)}$ ,

$$\mathbf{G}^{(i)} = \left( -\frac{1}{N} \sum_{n=1}^N \frac{\partial^2 \ln f_i(x_n, y_n | \boldsymbol{\theta}^{(i)})}{\partial \theta_{ik}^{(i)} \partial \theta_{il}^{(i)}} \bigg|_{\boldsymbol{\theta}^{(i)} = \hat{\boldsymbol{\theta}}_N^{(i)}} \right)_{kl}. \quad (\text{S-6})$$

Plugging this expression into Equation (10) of the manuscript yields

$$\mathfrak{B}_{\text{lnr}}(\mathcal{X}, \mathcal{Y} | D) = \ln \frac{L_1(\hat{\boldsymbol{\theta}}_N^{(1)})}{L_0(\hat{\boldsymbol{\theta}}_N^{(0)})} - \frac{D_2 - D_1}{2} \ln N + O(1). \quad (\text{S-7})$$

We now define

$$J_N(D) = \frac{1}{N} \sum_{n=1}^N \ln \frac{f_{XY}^{(1)}(\mathbf{x}_n, \mathbf{y}_n | \hat{\boldsymbol{\theta}}_N^{(1)})}{f_X^{(0)}(\mathbf{x}_n | \hat{\boldsymbol{\theta}}_N^{(0)}) f_Y^{(0)}(\mathbf{y}_n | \hat{\boldsymbol{\theta}}_N^{(0)})}, \quad (\text{S-8})$$

so that

$$\mathfrak{B}_{\text{lnr}}(\mathcal{X}, \mathcal{Y} | D) = N J_N(D) - \frac{D_1 - D_0}{2} \ln N + O(1). \quad (\text{S-9})$$

$J_N(D)$  can be further expressed as

$$J_N(D) = \frac{1}{N} \sum_{n=1}^N \ln \frac{f_{XY}^{(1)}(\mathbf{x}_n, \mathbf{y}_n | \hat{\boldsymbol{\theta}}_N^{(1)})}{f_X^{(1)}(\mathbf{x}_n | \hat{\boldsymbol{\theta}}_N^{(1)}) f_Y^{(1)}(\mathbf{y}_n | \hat{\boldsymbol{\theta}}_N^{(1)})} + \frac{1}{N} \sum_{n=1}^N \ln \frac{f_X^{(1)}(\mathbf{x}_n | \hat{\boldsymbol{\theta}}_N^{(1)})}{f_X^{(0)}(\mathbf{x}_n | \hat{\boldsymbol{\theta}}_N^{(0)})} + \frac{1}{N} \sum_{n=1}^N \ln \frac{f_Y^{(1)}(\mathbf{y}_n | \hat{\boldsymbol{\theta}}_N^{(1)})}{f_Y^{(0)}(\mathbf{y}_n | \hat{\boldsymbol{\theta}}_N^{(0)})}. \quad (\text{S-10})$$

The first term of the right-hand side is the sampling mutual information  $\hat{I}(X, Y)$  under  $H_1$ , leading to

$$\mathfrak{B}_{\text{lnr}}(\mathcal{X}, \mathcal{Y} | D) = N \left[ \hat{I}(X, Y) + \frac{1}{N} \sum_{n=1}^N \ln \frac{f_X^{(1)}(\mathbf{x}_n | \hat{\boldsymbol{\theta}}_N^{(1)})}{f_X^{(0)}(\mathbf{x}_n | \hat{\boldsymbol{\theta}}_N^{(0)})} + \frac{1}{N} \sum_{n=1}^N \ln \frac{f_Y^{(1)}(\mathbf{y}_n | \hat{\boldsymbol{\theta}}_N^{(1)})}{f_Y^{(0)}(\mathbf{y}_n | \hat{\boldsymbol{\theta}}_N^{(0)})} \right] - \frac{D_2 - D_1}{2} \ln N + O(1). \quad (\text{S-11})$$

### 3 Nested models

It can be shown (O'Hagan and Forster, 2004, §7.25) that  $2N J_N(D)$  (i.e., twice the likelihood ratio test statistic) is asymptotically distributed as a noncentral chi-square with  $D_2 - D_1$  degrees of freedom and noncentrality parameter  $N\lambda$  with

$$\lambda = (\boldsymbol{\phi} - \boldsymbol{\phi}_0)^t \mathbf{V}_{\boldsymbol{\phi}}^{-1} (\boldsymbol{\phi} - \boldsymbol{\phi}_0), \quad (\text{S-12})$$

where  $\mathbf{V}_{\boldsymbol{\phi}}$  derives from the information matrix of a single observation. The expectation of this quantity is therefore asymptotically equal to  $D_2 - D_1 + N\lambda$  and the variance twice this value.

Under  $H_0$ ,  $\lambda = 0$  (since  $\boldsymbol{\phi} = \boldsymbol{\phi}_0$ ), so that  $2N J_N(D)$  is a standard chi-square variable with  $D_2 - D_1$  degrees of freedom. According to Equation (S-9), Bienaymé–Chebyshev inequality entails that

$$\left( -\frac{D_1 - D_0}{2} \ln N \right)^{-1} \mathfrak{B}_{\text{lnr}}(\mathcal{X}, \mathcal{Y} | D) \quad (\text{S-13})$$

tends to 1 in probability as  $N \rightarrow \infty$ . This shows that, when  $N \rightarrow \infty$ ,  $\mathfrak{B}_{\text{lnr}}(\mathcal{X}, \mathcal{Y} | D)$  essentially behaves as  $-\frac{D_1 - D_0}{2} \ln N$ , which is a decreasing function of  $N$  that tends to  $-\infty$ . Also,  $\mathbb{E}[2N J_N(D)] = D_1 - D_0$ , so that

$$\mathbb{E}[\mathfrak{B}_{\text{lnr}}(\mathcal{X}, \mathcal{Y} | D) | H_0] = -\frac{D_1 - D_0}{2} \ln N + O(1), \quad (\text{S-14})$$

which is a decreasing function of  $N$ .

By contrast, under  $H_1$ ,  $\lambda > 0$ , so that Equation (S-9) and Bienaymé–Chebyshev inequality yield that

$$\left( \frac{N\lambda}{2} \right)^{-1} \mathfrak{B}_{\text{lnr}}(\mathcal{X}, \mathcal{Y} | D) \quad (\text{S-15})$$

tends to 1 in probability as  $N \rightarrow \infty$ , i.e.,  $\mathfrak{B}_{\text{lnr}}(\mathcal{X}, \mathcal{Y} | D)$  essentially behaves as  $N\lambda/2$ , which is an increasing function of  $N$  with limit  $+\infty$ . In this case,  $\mathbb{E}[2N J_N(D)] = N\lambda + D_2 - D_1$ , leading to

$$\mathbb{E}[\mathfrak{B}_{\text{lnr}}(\mathcal{X}, \mathcal{Y} | D) | H_1] = \frac{N\lambda}{2} - \frac{D_1 - D_0}{2} \ln N + O(1). \quad (\text{S-16})$$

While the first-order approximation is an increasing function of  $N$ , this second-order approximation may not be monotonic anymore. Indeed, if  $N_0 = (D_1 - D_2)/\lambda \geq 2$ , then  $\mathfrak{B}(\mathcal{X}, \mathcal{Y} | D)$  is decreasing for  $N \leq N_0$  and increasing for  $N \geq N_0$ .

## 4 Maximum-entropy distributions

### 4.1 Summary of results

We here delve in the particular case of maximum-entropy distributions (Jaynes, 2003, Chap. 11). We say that  $f(\mathbf{z}|\boldsymbol{\theta})$  with  $\boldsymbol{\theta} = (\theta_1, \dots, \theta_K)$  is a maximum-entropy distribution if there exists  $K$  functions  $u_k(\mathbf{z})$  and  $K$  values  $U_k$ ,  $1 \leq k \leq K$ , such that  $f(\mathbf{z}|\boldsymbol{\theta})$  maximizes entropy under the following constraints

$$\mathbb{E}[u_k(\mathbf{z})] = U_k, \quad 1 \leq k \leq K. \quad (\text{S-17})$$

One can show that such a distribution is of the form (Jaynes, 2003, Chap. 11)

$$f(\mathbf{z}|\boldsymbol{\theta}) = \frac{1}{Z(\boldsymbol{\theta})} \exp \left[ - \sum_{k=1}^K \theta_k u_k(\mathbf{z}) \right].$$

Maximum-entropy distributions are tightly related to exponential families (Bernardo and Smith, 2000, §4.5.3 and §4.5.4; Abramovich and Ritov, 2013, §1.6) or Koopman–Darmois families. Multivariate normal distributions and bivariate discrete distributions belong to this family.

For maximum-entropy distributions, it can be shown that for any  $\boldsymbol{\theta}^{(1)} \in \Theta^{(1)}$ , we have (Kullback, 1968, Chap. 5, §4; see also §4.2 below)

$$\ln \frac{L_1(\hat{\boldsymbol{\theta}}_N^{(1)})}{L_1(\boldsymbol{\theta}^{(1)})} = N D_{\text{KL}} \left[ f_{XY}^{(1)}(\mathbf{x}, \mathbf{y}|\hat{\boldsymbol{\theta}}_N^{(1)}) \| f_{XY}^{(1)}(\mathbf{x}, \mathbf{y}|\boldsymbol{\theta}^{(1)}) \right].$$

In the case where  $H_0$  is nested in  $H_1$ , we have

$$f_X^{(0)}(\mathbf{x}|\hat{\boldsymbol{\theta}}_N^{(0)}) f_Y^{(0)}(\mathbf{y}|\hat{\boldsymbol{\theta}}_N^{(0)}) = f_{XY}^{(1)} \left[ \mathbf{x}, \mathbf{y} | \pi(\hat{\boldsymbol{\theta}}_N^{(0)}) \right],$$

leading to

$$\begin{aligned} \ln \frac{L_1(\hat{\boldsymbol{\theta}}_N^{(1)})}{L_0(\hat{\boldsymbol{\theta}}_N^{(0)})} &= \ln \frac{L_1(\hat{\boldsymbol{\theta}}_N^{(1)})}{L_1 \left[ \pi(\hat{\boldsymbol{\theta}}_N^{(0)}) \right]} \\ &= N D_{\text{KL}} \left\{ f_{XY}^{(1)}(\mathbf{x}, \mathbf{y}|\hat{\boldsymbol{\theta}}_N^{(1)}) \| f_{XY}^{(1)} \left[ \mathbf{x}, \mathbf{y} | \pi(\hat{\boldsymbol{\theta}}_N^{(0)}) \right] \right\} \\ &= N D_{\text{KL}} \left[ f_{XY}^{(1)}(\mathbf{x}, \mathbf{y}|\hat{\boldsymbol{\theta}}_N^{(1)}) \| f_X^{(0)}(\mathbf{x}|\hat{\boldsymbol{\theta}}_N^{(0)}) f_Y^{(0)}(\mathbf{y}|\hat{\boldsymbol{\theta}}_N^{(0)}) \right]. \end{aligned} \quad (\text{S-18})$$

In our particular case, the Kullback–Leibler divergence is nothing else than mutual information and the right-hand side of Equation (S-18) the plug-in estimator for mutual information, so that

$$\mathfrak{B}_{\text{lnr}}(\mathcal{X}, \mathcal{Y}|D) = N \hat{I}(X, Y) - \frac{(D_1 - D_0)}{2} \ln N + O(1). \quad (\text{S-19})$$

This shows the connection of our approach with Kullback’s minimum discrimination information for the independence of  $X$  and  $Y$  (Kullback, 1968), as well as the connection with the BIC correction (Schwarz, 1978). See the particular cases of multivariate normal distributions and bivariate discrete distributions below, §5 and §6, respectively.

### 4.2 Intermediary results

**Definition and key properties.** Since  $\boldsymbol{\theta} = (\theta_1, \dots, \theta_K)$  is such that the  $K$  constraints of Equation (S-17) are respected, we obtain the following relationship between  $\theta_k$  and  $U_k$

$$\frac{\partial \ln Z(\boldsymbol{\theta})}{\partial \theta_k} = -U_k, \quad k = 1, \dots, K.$$

**Kullback–Leibler divergence.** Consider two maximum-entropy distributions  $f(\mathbf{z}|\boldsymbol{\theta})$  and  $f(\mathbf{z}|\boldsymbol{\theta}')$ , corresponding to expected values of  $u_k(\mathbf{z})$  equal to  $U_k$  and  $U'_k$ , respectively. We compute the Kullback–Leibler divergence from  $f(\mathbf{z}|\boldsymbol{\theta})$  to  $f(\mathbf{z}|\boldsymbol{\theta}')$

$$\begin{aligned} D[f(\mathbf{z}|\boldsymbol{\theta})||f(\mathbf{z}|\boldsymbol{\theta}')] &= \int f(\mathbf{z}|\boldsymbol{\theta}) \ln \frac{f(\mathbf{z}|\boldsymbol{\theta})}{f(\mathbf{z}|\boldsymbol{\theta}')} d\mathbf{z} \\ &= \int f(\mathbf{z}|\boldsymbol{\theta}) \ln f(\mathbf{z}|\boldsymbol{\theta}) d\mathbf{z} - \int f(\mathbf{z}|\boldsymbol{\theta}) \ln f(\mathbf{z}|\boldsymbol{\theta}') d\mathbf{z}, \end{aligned}$$

with

$$\int f(\mathbf{z}|\boldsymbol{\theta}) \ln f(\mathbf{z}|\boldsymbol{\theta}) d\mathbf{z} = -\ln Z(\boldsymbol{\theta}) - \sum_{k=1}^K \theta_k U_k$$

and

$$\int f(\mathbf{z}|\boldsymbol{\theta}) \ln f(\mathbf{z}|\boldsymbol{\theta}') d\mathbf{z} = -\ln Z(\boldsymbol{\theta}') - \sum_{k=1}^K \theta'_k U_k,$$

leading to

$$D[f(\mathbf{z}|\boldsymbol{\theta}); f(\mathbf{z}|\boldsymbol{\theta}')] = -\ln \frac{Z(\boldsymbol{\theta})}{Z(\boldsymbol{\theta}')} - \sum_{k=1}^K (\theta_k - \theta'_k) U_k. \quad (\text{S-20})$$

**Maximum likelihood.** We now consider a likelihood function that is a maximum-entropy distribution. It can therefore be expressed as

$$\ln L(\boldsymbol{\theta}) = -N \left[ \ln Z(\boldsymbol{\theta}) + \sum_k \theta_k \overline{u_k(z_n)} \right],$$

where  $\overline{u_k(z_n)}$  is the sampling average of  $u_k(z)$ ,

$$\overline{u_k(z_n)} = \frac{1}{N} \sum_{n=1}^N u_k(z_n).$$

The maximum-likelihood estimate is obtained by canceling the first derivatives of  $\ln L(\boldsymbol{\theta})$  with respect to each  $\theta_k$ , leading to the following equations

$$\frac{\partial \ln Z(\hat{\boldsymbol{\theta}})}{\partial \theta_k} = -\overline{u_k(z_n)}, \quad k = 1, \dots, K.$$

The corresponding maximum-entropy distribution is then such that

$$\mathbb{E}[u_k(z)] = \overline{u_k(z_n)}, \quad k = 1, \dots, K,$$

that is, its moments are equal to their sample counterparts.

**Connection with Kullback–Leibler divergence.** We finally compute the following log-likelihood ratio

$$\begin{aligned} \ln \frac{L(\hat{\boldsymbol{\theta}})}{L(\boldsymbol{\theta})} &= -N \left[ \ln \frac{Z(\hat{\boldsymbol{\theta}})}{Z(\boldsymbol{\theta})} + \sum_k (\hat{\theta}_k - \theta_k) \overline{u_k(z_n)} \right] \\ &= N D[f(\mathbf{z}|\hat{\boldsymbol{\theta}})||f(\mathbf{z}|\boldsymbol{\theta})], \end{aligned}$$

by comparison with Equation (S-20), since the moments of  $f(\mathbf{z}|\hat{\boldsymbol{\theta}})$  are equal to  $\overline{u_k(z_n)}$ .

## 5 Multivariate normal distributions

### 5.1 Summary of results

We here provide the derivation of  $\mathfrak{B}_{\text{lnr}}(\mathcal{X}, \mathcal{Y}|D)$  in the case of a multivariate normal distribution. More details can be found in Marrelec et al. (2015), Marrelec and Giron (2021), as well as in §5.2 below.

Assume that  $\mathcal{X}$  and  $\mathcal{Y}$  are such that  $(X, Y)$  has a multivariate normal distribution, with dimension  $D = D_X + D_Y$ . Let  $\mathbf{S}$  be the  $D$ -by- $D$  sum-of-square matrix of  $(X, Y)$ . Under the current assumptions and with conjugate priors (the prior distribution for **sigma**, the covariance matrix for  $(X, Y)$ , is set as an inverse-Wishart distribution with  $n$  degrees of freedom and scale matrix  $\mathbf{L}$ ),  $p(\mathbf{S}|H_1)$  and  $p(\mathbf{S}|H_0)$  can be calculated in closed form, yielding

$$p(\mathbf{S}|H_0) = \frac{|\mathbf{S}|^{\frac{N-D-1}{2}}}{Z(D, N)} \prod_{k \in \{X, Y\}} \frac{Z(D_k, N + n_k)}{Z(D_k, n_k)} \frac{|\mathbf{L}_{kk}|^{\frac{n_k}{2}}}{|\mathbf{S}_{kk} + \mathbf{L}_{kk}|^{\frac{N+n_k}{2}}}$$

and

$$p(\mathbf{S}|H_1) = \frac{|\mathbf{S}|^{\frac{N-D-1}{2}}}{Z(D, N)} \frac{Z(D, N + n)}{Z(D, n)} \frac{|\mathbf{L}|^{\frac{n}{2}}}{|\mathbf{S} + \mathbf{L}|^{\frac{N+n}{2}}},$$

where  $\mathbf{S} + \mathbf{L}$  is the regularized sample sum-of-square matrix,  $\mathbf{S}_{kk}$  and  $\mathbf{L}_{kk}$  the subblocks of  $\mathbf{S}$  and  $\mathbf{L}$ , respectively, corresponding to  $k \in \{X, Y\}$ ,  $n_k = n - D + D_k$ , and  $Z(d, n)$  the inverse of a normalization constant

$$Z(d, n) = 2^{\frac{nd}{2}} \pi^{\frac{d(d-1)}{4}} \prod_{d'=1}^d \Gamma\left(\frac{n+1-d'}{2}\right).$$

$\Pr(H_0|\mathbf{S})$  and  $\Pr(H_1|\mathbf{S})$  can be computed directly from there using Bayes updating rule, Equation (4) of the manuscript. It can be shown that, asymptotically ( $N \rightarrow \infty$ ), we have

$$\mathfrak{B}_{\text{lnr}}(\mathcal{X}, \mathcal{Y}|D) = N\hat{I}(X, Y) - \frac{D_X D_Y}{2} \ln N + O(1), \quad (\text{S-21})$$

where

$$\hat{I}(X, Y) = \frac{1}{2} \ln \frac{|\hat{\mathbf{S}}_{XX}| |\hat{\mathbf{S}}_{YY}|}{|\hat{\mathbf{S}}|}$$

is the plug-in estimator of mutual information for a multivariate normal distribution, with  $\hat{\mathbf{S}}$  the sample covariance matrix. Alternatively,  $N\hat{I}(X, Y)$  is the minimum discrimination information for the independence of  $X$  and  $Y$  (Kullback, 1968, Chap. 12, §3.6). Alternatively,  $-N\hat{I}(X, Y)$  can also be seen as the log-likelihood ratio criterion (Anderson, 1958, §9.7). Also, in Equation (S-21), the term in log is the BIC correction for the number of parameters [ $D(D+1)/2$  in  $H_1$ , versus  $D_X(D_X+1)/2 + D_Y(D_Y+1)/2$  in  $H_0$ ].

In the particular case where  $(X, Y)$  is bivariate normal ( $D_X = D_Y = 1$ ), Equation (S-21) boils down to

$$\mathfrak{B}_{\text{lnr}}(\mathcal{X}, \mathcal{Y}|D) = -\frac{N}{2} \ln(1 - r^2) - \frac{1}{2} \ln N + O(1),$$

where  $r$  is the sample correlation coefficient between  $X$  and  $Y$  and

$$\hat{I}(X, Y) = -\frac{1}{2} \ln(1 - r^2), \quad (\text{S-22})$$

is again the plug-in estimator for mutual information. These results illustrate the connection between Bayesian model comparison, the log-likelihood ratio criterion, the plug-in estimate for mutual information, and the minimum discrimination information for the independence.

## 5.2 Intermediary results

**Marginal model likelihood under the hypothesis of dependence.** Let us first calculate  $p(\mathbf{S}|H_1)$ , the marginal model likelihood under the hypothesis of dependence. Expressing this quantity as a function of the model parameters yields

$$p(\mathbf{S}|H_1) = \int p(\mathbf{S}|H_1, \boldsymbol{\Sigma}^{(1)}) p(\boldsymbol{\Sigma}^{(1)}|H_1) d\boldsymbol{\Sigma}^{(1)}. \quad (\text{S-23})$$

Calculation of the integral requires to know the likelihood  $p(\mathbf{S}|H_1, \boldsymbol{\Sigma}^{(1)})$  and the prior distribution  $p(\boldsymbol{\Sigma}^{(1)}|H_1)$  of the covariance matrix under  $H_1$ . With multivariate normal data,  $\mathbf{S}$  given  $\boldsymbol{\Sigma}^{(1)}$  is Wishart distributed with  $N$  degrees of freedom and scale matrix  $\boldsymbol{\Sigma}^{(1)}$  (Anderson, 2003, Corollary 7.2.2), leading to the following likelihood

$$p(\mathbf{S}|H_1, \boldsymbol{\Sigma}^{(1)}) = \frac{|\mathbf{S}|^{\frac{N-D-1}{2}}}{Z(D, N)} |\boldsymbol{\Sigma}^{(1)}|^{-\frac{N}{2}} \exp \left\{ -\frac{1}{2} \text{tr} \left[ (\boldsymbol{\Sigma}^{(1)})^{-1} \mathbf{S} \right] \right\}, \quad (\text{S-24})$$

where  $Z(d, n)$  is the inverse of the normalization constant

$$Z(d, n) = 2^{\frac{nd}{2}} \pi^{\frac{d(d-1)}{4}} \prod_{d'=1}^d \Gamma \left( \frac{n+1-d'}{2} \right).$$

As to the prior distribution, this quantity is here set as a conjugate prior, namely an inverse-Wishart distribution with  $n$  degrees of freedom and scale matrix  $\mathbf{L}$  (Gelman et al., 2004, §3.6)

$$p(\boldsymbol{\Sigma}^{(1)}|H_1) = \frac{|\mathbf{L}|^{\frac{n}{2}}}{Z(D, n)} |\boldsymbol{\Sigma}^{(1)}|^{-\frac{n+D+1}{2}} \exp \left\{ -\frac{1}{2} \text{tr} \left[ (\boldsymbol{\Sigma}^{(1)})^{-1} \mathbf{L} \right] \right\}. \quad (\text{S-25})$$

Bringing Equations (S-24) and (S-25) together into Equation (S-23) yields for the marginal model likelihood

$$p(\mathbf{S}|H_1) = \frac{|\mathbf{L}|^{\frac{n}{2}} |\mathbf{S}|^{\frac{N-D-1}{2}}}{Z(D, N) Z(D, n)} \int |\boldsymbol{\Sigma}^{(1)}|^{-\frac{N+n+D+1}{2}} \exp \left\{ -\frac{1}{2} \text{tr} \left[ (\mathbf{L} + \mathbf{S})(\boldsymbol{\Sigma}^{(1)})^{-1} \right] \right\} d\boldsymbol{\Sigma}^{(1)}.$$

The integrand is proportional to an inverse-Wishart distribution with  $N+n$  degrees of freedom and scale matrix  $\mathbf{L} + \mathbf{S}$ , leading to

$$p(\mathbf{S}|H_1) = \frac{|\mathbf{S}|^{\frac{N-D-1}{2}}}{Z(D, N)} \frac{Z(D, N+n)}{Z(D, n)} \frac{|\mathbf{L}|^{\frac{n}{2}}}{|\mathbf{S} + \mathbf{L}|^{\frac{N+n}{2}}}. \quad (\text{S-26})$$

**Marginal model likelihood under the hypothesis of independence.** We can now calculate  $P(\mathbf{S}|H_0)$ , the marginal model likelihood under the hypothesis of independence. If  $H_0$  holds, then  $\boldsymbol{\Sigma}^{(0)}$  is block-diagonal with two blocks  $\boldsymbol{\Sigma}_{XX}^{(0)}$  and  $\boldsymbol{\Sigma}_{YY}^{(0)}$  the submatrix restrictions of  $\boldsymbol{\Sigma}^{(0)}$  to  $\mathbf{X}$  and  $\mathbf{Y}$ , respectively. Introduction of the model parameters therefore yields for the marginal likelihood

$$p(\mathbf{S}|H_0) = \int p(\mathbf{S}|H_0, \boldsymbol{\Sigma}_{XX}^{(0)}, \boldsymbol{\Sigma}_{YY}^{(0)}) p(\boldsymbol{\Sigma}_{XX}^{(0)}, \boldsymbol{\Sigma}_{YY}^{(0)}|H_0) d\boldsymbol{\Sigma}_{XX}^{(0)} d\boldsymbol{\Sigma}_{YY}^{(0)}. \quad (\text{S-27})$$

To calculate this integral, we again need to know the likelihood  $p(\mathbf{S}|H_0, \boldsymbol{\Sigma}_{XX}^{(0)}, \boldsymbol{\Sigma}_{YY}^{(0)})$  and the prior distribution  $p(\boldsymbol{\Sigma}_{XX}^{(0)}, \boldsymbol{\Sigma}_{YY}^{(0)}|H_0)$  of the two blocks of the covariance matrix under  $H_0$ . The likelihood is the same as for  $H_0$  and has the form of Equation (S-24). Furthermore, since  $\boldsymbol{\Sigma}^{(0)}$  is here block diagonal, we have  $|\boldsymbol{\Sigma}| = |\boldsymbol{\Sigma}_{XX}^{(0)}| |\boldsymbol{\Sigma}_{YY}^{(0)}|$  and  $\text{tr}[(\boldsymbol{\Sigma}^{(0)})^{-1} \mathbf{S}] = \text{tr}[(\boldsymbol{\Sigma}_{XX}^{(0)})^{-1} \mathbf{S}_{XX}] + \text{tr}[(\boldsymbol{\Sigma}_{YY}^{(0)})^{-1} \mathbf{S}_{YY}]$ , where  $\mathbf{S}_{XX}$  and  $\mathbf{S}_{YY}$  are the restrictions of  $\mathbf{S}$  to  $\mathbf{X}$  and  $\mathbf{Y}$ , respectively. Consequently, the likelihood can be further expanded as

$$p(\mathbf{S}|H_0, \boldsymbol{\Sigma}_{XX}^{(0)}, \boldsymbol{\Sigma}_{YY}^{(0)}) = \frac{|\mathbf{S}|^{\frac{N-D-1}{2}}}{Z(D, N)} \prod_{k=X,Y} |\boldsymbol{\Sigma}_{kk}^{(0)}|^{-\frac{N}{2}} \exp \left\{ -\frac{1}{2} \text{tr} \left[ (\boldsymbol{\Sigma}_{kk}^{(0)})^{-1} \mathbf{S}_{kk} \right] \right\}. \quad (\text{S-28})$$

As to the prior distribution, assuming no prior dependence between  $\boldsymbol{\Sigma}_{XX}^{(0)}$  and  $\boldsymbol{\Sigma}_{YY}^{(0)}$  yields

$$p(\boldsymbol{\Sigma}_{XX}^{(0)}, \boldsymbol{\Sigma}_{YY}^{(0)} | H_0) = p(\boldsymbol{\Sigma}_{XX}^{(0)} | H_0) p(\boldsymbol{\Sigma}_{YY}^{(0)} | H_0). \quad (\text{S-29})$$

For the sake of consistency,  $p(\boldsymbol{\Sigma}_{XX}^{(0)} | H_0)$  and  $p(\boldsymbol{\Sigma}_{YY}^{(0)} | H_0)$  are set equal to  $p(\boldsymbol{\Sigma}_{XX}^{(1)} | H_1)$  and  $p(\boldsymbol{\Sigma}_{YY}^{(1)} | H_1)$ , respectively, which are in turn obtained by marginalization of  $p(\boldsymbol{\Sigma}^{(1)} | H_1)$  as given by Equation (S-25). For  $k \in \{X, Y\}$ ,  $p(\boldsymbol{\Sigma}_{kk}^{(0)} | H_0)$  can be found to have an inverse-Wishart distribution with  $n_k = n - D + D_k$  degrees of freedom and scale matrix  $\mathbf{L}_k$  the restriction of  $\mathbf{L}$  to  $k$  (Press, 2005, §5.2)

$$p(\boldsymbol{\Sigma}_{kk}^{(0)} | H_0) = \frac{|\mathbf{L}_{kk}|^{\frac{n}{2}}}{Z(D_k, n_k)} |\boldsymbol{\Sigma}_{kk}^{(0)}|^{-\frac{n_k + D_k + 1}{2}} \exp \left\{ -\frac{1}{2} \text{tr} \left[ \mathbf{L}_k (\boldsymbol{\Sigma}_{kk}^{(0)})^{-1} \right] \right\}. \quad (\text{S-30})$$

Incorporating Equations (S-28), (S-29), and (S-30) into Equation (S-27) yields

$$p(\mathbf{S} | H_0) = \frac{|\mathbf{S}|^{\frac{N-D-1}{2}}}{Z(D, N)} \prod_{k=X,Y} \frac{|\mathbf{L}_{kk}|^{\frac{n_k}{2}}}{Z(D_k, n_k)} \int |\boldsymbol{\Sigma}_{kk}^{(0)}|^{-\frac{N+n_k+D_k+1}{2}} \exp \left\{ -\frac{1}{2} \text{tr} \left[ (\mathbf{S}_k + \mathbf{L}_k) (\boldsymbol{\Sigma}_{kk}^{(0)})^{-1} \right] \right\}.$$

Each integrand is proportional to an inverse-Wishart distribution with  $N + n_k$  degrees of freedom and scale matrix  $\mathbf{S}_{kk} + \mathbf{L}_{kk}$ , leading to

$$p(\mathbf{S} | H_0) = \frac{|\mathbf{S}|^{\frac{N-D-1}{2}}}{Z(D, N)} \prod_{k=X,Y} \frac{Z(D_k, N + n_k)}{Z(D_k, n_k)} \frac{|\mathbf{L}_{kk}|^{\frac{n_k}{2}}}{|\mathbf{S}_{kk} + \mathbf{L}_{kk}|^{\frac{N+n_k}{2}}}. \quad (\text{S-31})$$

**Asymptotic form of the log Bayes factor.** From Equations (S-26) and (S-31), we have

$$\begin{aligned} \ln \frac{p(\mathbf{S} | H_1)}{p(\mathbf{S} | H_0)} &= \sum_{d=1}^D \ln \Gamma \left( \frac{N + n + 1 - d}{2} \right) - \frac{N + n}{2} \ln |\mathbf{S} + \mathbf{L}| \\ &\quad - \sum_{k \in \{X, Y\}} \left[ \sum_{d=1}^{D_k} \ln \Gamma \left( \frac{N + n_k + 1 - d}{2} \right) - \frac{N + n_k}{2} \ln |\mathbf{S}_{kk} + \mathbf{L}_{kk}| \right] + O(1). \end{aligned}$$

In the following, we consider  $k \in \{X, Y, (X, Y)\}$ , with the convention that  $\mathbf{S}_{(X,Y)} = \mathbf{S}$ , etc. For the Gamma functions, we apply Stirling approximation (Abramowitz and Stegun, 1972, p. 257)

$$\ln \Gamma(z) = \left( z - \frac{1}{2} \right) \ln z - z + O(1).$$

Setting  $z = (N + n_k + 1 - d)/2$ , we obtain

$$\ln \Gamma \left( \frac{N + n_k + 1 - d}{2} \right) = \frac{N + n_k - d}{2} \ln N - \frac{N}{2} (1 + \ln 2) + O(1).$$

Summing this expression over  $d = 1, \dots, D_k$  and using the fact that  $\sum_{d=1}^{D_k} d = D_k(D_k + 1)/2$  leads us to

$$\sum_{d=1}^{D_k} \ln \Gamma \left( \frac{N + n_k + 1 - d}{2} \right) = D_k \left[ \frac{N + n_k}{2} \ln N - \frac{N}{2} (1 + \ln 2) \right] - \frac{D_k(D_k + 1)}{4} \ln N + O(1). \quad (\text{S-32})$$

Defining  $\hat{\mathbf{S}}_{kk}$  as the standard sample covariance matrix, i.e.,  $\mathbf{S}_{kk} = N \hat{\mathbf{S}}_{kk}$ , each log term can be expanded as

$$\begin{aligned} \frac{N + n_k}{2} \ln |\mathbf{S}_{kk} + \mathbf{L}_{kk}| &= \frac{N + n_k}{2} \ln |N \hat{\mathbf{S}}_{kk} + \mathbf{L}_{kk}| \\ &= \left( \frac{N}{2} + \frac{n_k}{2} \right) \left[ D_k \ln N + \ln |\hat{\mathbf{S}}_{kk}| + \ln |\mathbf{I} + (N \hat{\mathbf{S}}_{kk})^{-1} \mathbf{L}_{kk}| \right] \\ &= \frac{D_k N}{2} \ln N + \frac{N}{2} \ln |\hat{\mathbf{S}}_{kk}| + \frac{D_k n_k}{2} \ln N + O(1), \end{aligned}$$

since  $|a\mathbf{A}| = a^{\dim(\mathbf{A})}|\mathbf{A}|$  for any positive number  $a$  and matrix  $\mathbf{A}$ . We therefore have

$$\begin{aligned} & \sum_{d=1}^{D_k} \ln \Gamma \left( \frac{N + n_k + 1 - d}{2} \right) - \frac{N + n_k}{2} \ln |\mathbf{S}_{kk} + \mathbf{L}_{kk}| \\ &= -\frac{D_k N}{2} (1 + \ln 2) - \frac{D_k(D_k + 1)}{4} \ln N - \frac{N}{2} \ln |\hat{\mathbf{S}}_{kk}| + O(1). \end{aligned}$$

Finally, putting all results together, we obtain

$$\begin{aligned} \ln \frac{p(\mathbf{S}|H_1)}{p(\mathbf{S}|H_0)} &= \frac{N}{2} \ln \frac{|\hat{\mathbf{S}}_{XX}| |\hat{\mathbf{S}}_{YY}|}{|\hat{\mathbf{S}}|} - \frac{1}{2} \left[ \frac{D(D+1)}{2} - \sum_{k \in \{X, Y\}} \frac{D_k(D_k+1)}{2} \right] \ln N + O(1) \\ &= \frac{N}{2} \ln \frac{|\hat{\mathbf{S}}_{XX}| |\hat{\mathbf{S}}_{YY}|}{|\hat{\mathbf{S}}|} - \frac{D_X D_Y}{2} \ln N + O(1). \end{aligned}$$

## 6 Bivariate discrete distributions

### 6.1 Summary of results

The same work can be done in the case of a bivariate discrete distribution, showing the relationship between Bayesian model comparison and discrete mutual information (Wolf, 1994; Marrelec and Giron, 2021). For more details regarding the calculations, the reader can refer to 6.2 below.

Consider two discrete variables  $X$  and  $Y$  taking  $r$  and  $s$  values respectively, such that

$$p(X = x_i, Y = y_j) = \theta_{ij}, \quad i = 1, \dots, r, \quad j = 1, \dots, s.$$

The dataset is composed of the number of observations  $N_{ij}$  for which  $X = x_i$  and  $Y = y_j$ . We set  $N_{i\cdot} = \sum_j N_{ij}$ ,  $N_{\cdot j} = \sum_i N_{ij}$  and  $N = \sum_{ij} N_{ij}$ . Using a conjugate prior for  $\boldsymbol{\theta} = (\theta_{ij})$  (i.e., a Dirichlet prior with parameters  $a_{ij}$ ), the marginal model likelihoods are given by

$$p(D|H_0) = \frac{\Gamma(a)}{\prod_i \Gamma(a_{i\cdot})} \frac{\prod_i \Gamma(N_{i\cdot} + a_{i\cdot})}{\Gamma(N + a)} \frac{\Gamma(a)}{\prod_j \Gamma(a_{\cdot j})} \frac{\prod_j \Gamma(N_{\cdot j} + a_{\cdot j})}{\Gamma(N + a)}$$

and

$$p(D|H_1) = \frac{\Gamma(a)}{\prod_{i,j} \Gamma(a_{ij})} \frac{\prod_{i,j} \Gamma(N_{ij} + a_{ij})}{\Gamma(N + a)},$$

respectively, where we also set  $a_{i\cdot} = \sum_j a_{ij}$ ,  $a_{\cdot j} = \sum_i a_{ij}$  and  $a = \sum_{ij} a_{ij}$ . Set  $N_{ij} = f_{ij}N$  the observed frequencies, together with  $N_{i\cdot} = f_{i\cdot}N$  and  $N_{\cdot j} = f_{\cdot j}N$  their marginal counterparts. When  $N \rightarrow \infty$ , use of Stirling approximation (Abramowitz and Stegun, 1972, p. 257) leads to

$$\mathfrak{B}_{\text{lnr}}(\mathcal{X}, \mathcal{Y}|D) = N \sum_{ij} f_{ij} \ln \frac{f_{ij}}{f_{i\cdot} f_{\cdot j}} - \frac{(rs - 1) - (r - 1) - (s - 1)}{2} \ln N + O(1).$$

Again, we see the plug-in estimator of mutual information in the case of bivariate normal distributions

$$\hat{I}(X, Y) = \sum_{ij} f_{ij} \ln \frac{f_{ij}}{f_{i\cdot} f_{\cdot j}}$$

as well as a BIC correction for the number of parameters [ $rs - 1$  in  $H_1$ , versus  $(r - 1) + (s - 1)$  in  $H_0$ ]. This allows us to express  $\mathfrak{B}_{\text{lnr}}(\mathcal{X}, \mathcal{Y}|D)$  as

$$\mathfrak{B}_{\text{lnr}}(\mathcal{X}, \mathcal{Y}|D) = N \hat{I}(X, Y) - \frac{(r - 1)(s - 1)}{2} \ln N + O(1). \quad (\text{S-33})$$

Note that  $2N\hat{I}(X, Y)$  is equal to the deviance and is closely related to Pearson's chi-squared statistic for the goodness of fit (Whittaker, 1990, §7.4; Wolf, 1994).

## 6.2 Intermediary results

**Marginal model likelihood under the hypothesis of dependence.** Setting  $\boldsymbol{\theta}^{(1)} = (\theta_{ij}^{(1)})$ , we have

$$p(D|H_1) = \int p(\boldsymbol{\theta}^{(1)}|H_1) p(D|H_1, \boldsymbol{\theta}^{(1)}) d\boldsymbol{\theta}^{(1)}.$$

We set a Dirichlet distribution with parameters  $\mathbf{a} = (a_{ij})$  for  $\boldsymbol{\theta}^{(1)}$  such that  $\sum_{ij} \theta_{ij}^{(1)} = 1$ ,

$$p(\boldsymbol{\theta}^{(1)}) = \frac{\Gamma\left(\sum_{ij} a_{ij}\right)}{\prod_{i,j} \Gamma(a_{ij})} (\theta_{ij}^{(1)})^{a_{ij}}.$$

Besides, the likelihood reads

$$p(D|H_1, \boldsymbol{\theta}) = \prod_{i,j} (\theta_{ij}^{(1)})^{N_{ij}},$$

where  $N_{ij}$  is the number of time that we observe the pair  $(x_i, y_j)$ . The marginal model likelihood thus yields

$$p(D|H_1) = \frac{\Gamma\left(\sum_{ij} a_{ij}\right)}{\prod_{i,j} \Gamma(a_{ij})} \int \prod_{i,j} (\theta_{ij}^{(1)})^{N_{ij}+a_{ij}} d\boldsymbol{\theta}^{(1)}.$$

As a function of  $\boldsymbol{\theta}^{(1)}$ , this expression is proportional to a Dirichlet distribution with parameters  $N_{ij} + a_{ij}$ . Integration with respect to  $\boldsymbol{\theta}^{(1)}$  therefore yields

$$p(D|H_1) = \frac{\Gamma(a)}{\prod_{i,j} \Gamma(a_{ij})} \frac{\prod_{i,j} \Gamma(N_{ij} + a_{ij})}{\Gamma(N + a)}, \quad (\text{S-34})$$

where we set  $a = \sum_{ij} a_{ij}$ .

**Marginal model likelihood under the hypothesis of independence.** We now focus on  $p(D|H_0)$ , which can be expressed as

$$p(D|H_0) = \int p(\boldsymbol{\phi}^{(0)}, \boldsymbol{\psi}^{(0)}|H_0) p(D|H_0, \boldsymbol{\phi}^{(0)}, \boldsymbol{\psi}^{(0)}) d\boldsymbol{\phi}^{(0)} d\boldsymbol{\psi}^{(0)},$$

where we set  $\boldsymbol{\phi}^{(0)} = (\phi_i^{(0)})$  and  $\boldsymbol{\psi}^{(0)} = (\psi_j^{(0)})$ , with  $p(X = x_i) = \phi_i^{(0)}$  and  $p(Y = y_j) = \psi_j^{(0)}$ . We again set Dirichlet distributions for  $\boldsymbol{\phi}^{(0)}$  and  $\boldsymbol{\psi}^{(0)}$ . Since each  $\phi_i^{(0)}$  can be obtained as

$$\phi_i^{(0)} = \sum_j \theta_{ij}^{(1)},$$

consistency imposes that the prior for each  $\phi_i^{(0)}$  be equal to the prior for  $\sum_j \theta_{ij}^{(1)}$  in  $H_1$ , yielding

$$p(\boldsymbol{\phi}^{(0)}) = \frac{\Gamma(a)}{\prod_i \Gamma(a_{i\cdot})} \prod_i (\phi_i^{(0)})^{a_{i\cdot}},$$

where we set  $a_{i\cdot} = \sum_j a_{ij}$ . Similarly for  $\boldsymbol{\psi}^{(0)}$ ,

$$p(\boldsymbol{\psi}^{(0)}) = \frac{\Gamma(a)}{\prod_j \Gamma(a_{\cdot j})} \prod_j (\psi_j^{(0)})^{a_{\cdot j}},$$

with  $a_{\cdot j} = \sum_i a_{ij}$ . Besides, the likelihood reads

$$p(D|H_0, \boldsymbol{\phi}^{(0)}, \boldsymbol{\psi}^{(0)}) = \prod_i (\phi_i^{(0)})^{N_{i\cdot}} \prod_j (\psi_j^{(0)})^{N_{\cdot j}},$$

with  $N_{i\cdot} = \sum_j N_{ij}$  and  $N_{\cdot j} = \sum_i N_{ij}$ . The marginal model likelihood thus yields

$$p(D|H_0) = \frac{\Gamma(a)}{\prod_i \Gamma(a_{i\cdot})} \frac{\Gamma(a)}{\prod_j \Gamma(a_{\cdot j})} \left[ \int \prod_i (\phi_i^{(0)})^{N_{i\cdot} + a_{i\cdot}} d\phi^{(0)} \right] \left[ \int \prod_j (\psi_j^{(0)})^{N_{\cdot j} + a_{\cdot j}} d\psi^{(0)} \right].$$

As a function of  $\phi$ , the first integrand is proportional to a Dirichlet distribution with parameters  $N_{i\cdot} + a_{i\cdot}$ , and similarly for the second integrand. Integration with respect to  $\phi^{(0)}$  and  $\psi^{(0)}$  therefore yields

$$p(D|H_0) = \frac{\Gamma(a)}{\prod_i \Gamma(a_{i\cdot})} \frac{\prod_i \Gamma(N_{i\cdot} + a_{i\cdot})}{\Gamma(N + a)} \frac{\Gamma(a)}{\prod_j \Gamma(a_{\cdot j})} \frac{\prod_j \Gamma(N_{\cdot j} + a_{\cdot j})}{\Gamma(N + a)}. \quad (\text{S-35})$$

**Asymptotic approximation.** From the expression of  $p(D|H_1)$ , Equation (S-34), we have

$$\ln p(D|H_1) = \sum_{ij} \ln \Gamma(N_{ij} + a_{ij}) - \ln \Gamma(N + a) + \text{cst},$$

where "cst" is a term that does not depend on the data. Set  $f_{ij} = N_{ij}/N$ , so that  $\sum_{ij} f_{ij} = 1$ . In the following, we assume large data set,  $N \rightarrow \infty$  and use the following approximation for the Gamma function (Abramowitz and Stegun, 1972, p. 257)

$$\ln \Gamma(z) = \left( z - \frac{1}{2} \right) \ln z - z + O(1).$$

We have

$$\begin{aligned} \ln \Gamma(N + a) &= \left( N + a - \frac{1}{2} \right) \ln(N + a) - (N + a) + O(1) \\ &= N \ln N - N + \left( a - \frac{1}{2} \right) \ln N + O(1) \end{aligned}$$

and, similarly,

$$\begin{aligned} \ln \Gamma(N_{ij} + a_{ij}) &= \ln \Gamma(f_{ij}N + a_{ij}) \\ &= \left( f_{ij}N + a_{ij} - \frac{1}{2} \right) \ln(f_{ij}N + a_{ij}) - (f_{ij}N + a_{ij}) + O(1) \\ &= f_{ij}N \ln N + N(f_{ij} \ln f_{ij} - f_{ij}) + \left( a_{ij} - \frac{1}{2} \right) \ln N + O(1). \end{aligned}$$

Putting these two results together yields

$$\ln p(D|H_1) = N \sum_{ij} f_{ij} \ln f_{ij} - \frac{rs - 1}{2} \ln N + O(1).$$

Similarly, for  $H_0$ , we obtain from Equation (S-35)

$$\ln p(D|H_0) = N \sum_i f_{i\cdot} \ln f_{i\cdot} - \frac{r - 1}{2} \ln N + N \sum_j f_{\cdot j} \ln f_{\cdot j} - \frac{s - 1}{2} \ln N + O(1).$$

Finally,

$$\ln \frac{p(D|H_1)}{p(D|H_0)} = N \sum_{ij} f_{ij} \ln \frac{f_{ij}}{f_{i\cdot} f_{\cdot j}} - \frac{(rs - 1) - (r - 1) - (s - 1)}{2} \ln N + O(1).$$

**Maximum-likelihood estimate.** For model  $H_1$ , the maximum-likelihood estimate is given by

$$\hat{\theta}_{ij} = \frac{N_{ij}}{N} = f_{ij}.$$

The corresponding maximum of the log-likelihood is then equal to

$$\ln p(D|H_1, \hat{\boldsymbol{\theta}}^{(1)}) = N \sum_{ij} f_{ij} \ln f_{ij},$$

which corresponds to the the first term in the right-hand side of the approximation of  $p(D|H_1)$ . Similarly, for model  $H_0$ , we have

$$\hat{\phi}_i^{(0)} = \frac{N_{i\cdot}}{N} = f_{i\cdot}$$

and

$$\hat{\psi}_j^{(0)} = \frac{N_{\cdot j}}{N} = f_{\cdot j},$$

so that

$$\ln p(D|H_0, \hat{\boldsymbol{\phi}}^{(0)}, \hat{\boldsymbol{\psi}}^{(0)}) = N \sum_{ij} f_{ij} \ln f_{ij},$$

which corresponds to the the first term in the right-hand side of the approximation of  $p(D|H_1)$ .

## 7 Model misspecification

We here consider the case of model misspecification, in the case of known distributions (7.1) and known likelihood functions with unknown parameters (7.2).

### 7.1 Known distributions

We first assume that the distributions are known (see 1). In this case, the likelihood function  $f(\mathbf{x}, \mathbf{y})$  is different from both  $f_X^{(0)}(\mathbf{x})f_Y^{(0)}(\mathbf{y})$  and  $f_{XY}^{(1)}(\mathbf{x}, \mathbf{y})$ . We can then express  $J_N(D)$  of Equation (S-2) as

$$J_N(D) = \frac{1}{N} \sum_{n=1}^N \ln \frac{f(\mathbf{x}_n, \mathbf{y}_n)}{f_X^{(0)}(\mathbf{x}_n) f_Y^{(0)}(\mathbf{y}_n)} - \frac{1}{N} \sum_{n=1}^N \ln \frac{f(\mathbf{x}_n, \mathbf{y}_n)}{f_{XY}^{(1)}(\mathbf{x}_n, \mathbf{y}_n)}.$$

According to the strong law of large numbers, the two sums tend to

$$\int f(\mathbf{x}, \mathbf{y}) \ln \frac{f(\mathbf{x}, \mathbf{y})}{f_X^{(0)}(\mathbf{x}) f_Y^{(0)}(\mathbf{y})} d\mathbf{x} d\mathbf{y} = D_{\text{KL}} \left[ f(\mathbf{x}, \mathbf{y}) \| f_X^{(0)}(\mathbf{x}) f_Y^{(0)}(\mathbf{y}) \right]$$

and

$$\int f(\mathbf{x}, \mathbf{y}) \ln \frac{f(\mathbf{x}, \mathbf{y})}{f_{XY}^{(1)}(\mathbf{x}, \mathbf{y})} d\mathbf{x} d\mathbf{y} = D_{\text{KL}} \left[ f(\mathbf{x}, \mathbf{y}) \| f_{XY}^{(1)}(\mathbf{x}, \mathbf{y}) \right],$$

respectively. This shows that

$$J_N(D) \xrightarrow{N \rightarrow \infty} D_{\text{KL}} \left[ f(\mathbf{x}, \mathbf{y}); f_X^{(0)}(\mathbf{x}) f_Y^{(0)}(\mathbf{y}) \right] - D_{\text{KL}} \left[ f(\mathbf{x}, \mathbf{y}) \| f_{XY}^{(1)}(\mathbf{x}, \mathbf{y}) \right].$$

$J_N(D)$  therefore tends to a negative value if  $H_0$  is closer to the true generative model (in the sense of Kullback–Leibler divergence), and to a positive value if it is  $H_1$  that is closer. According to Equation (S-3), for  $N$  large enough,  $\mathfrak{B}_{\text{lnr}}(\mathcal{X}, \mathcal{Y}|D)$  will therefore be a decreasing function of  $N$  with limit  $-\infty$  if  $H_0$  is closer to the true model, while it will be an increasing function of  $N$  with limit  $+\infty$  if it is  $H_1$  that is closer. In other words,  $\mathfrak{B}_{\text{lnr}}(\mathcal{X}, \mathcal{Y}|D)$  behaves as if the model closer to the true generative one were the true one.

## 7.2 Known likelihood functions with unknown parameters

$J_N(D)$  of Equation (S-8) yields

$$J_N(D) = \frac{1}{N} \sum_{n=1}^N \ln \frac{f(\mathbf{x}_n, \mathbf{y}_n | \boldsymbol{\theta})}{f_X^{(0)}(\mathbf{x}_n | \hat{\boldsymbol{\theta}}_N^{(0)}) f_Y^{(0)}(\mathbf{y}_n | \hat{\boldsymbol{\theta}}_N^{(0)})} - \frac{1}{N} \sum_{n=1}^N \ln \frac{f(\mathbf{x}_n, \mathbf{y}_n | \boldsymbol{\theta})}{f_{XY}^{(1)}(\mathbf{x}_n, \mathbf{y}_n | \hat{\boldsymbol{\theta}}_N^{(1)})}.$$

We now assume that the estimators have limits, i.e.,  $\hat{\boldsymbol{\theta}}_N^{(0)} \xrightarrow{N \rightarrow \infty} \boldsymbol{\theta}_\infty^{(0)}$  and  $\hat{\boldsymbol{\theta}}_N^{(1)} \xrightarrow{N \rightarrow \infty} \boldsymbol{\theta}_\infty^{(1)}$ , and that these limits are such that Laplace approximation of Equation (S-5) can be applied. In this case, the likelihood ratio test statistic can be further expanded as

$$\begin{aligned} J_N(D) = & \frac{1}{N} \sum_{n=1}^N \ln \frac{f(\mathbf{x}_n, \mathbf{y}_n | \boldsymbol{\theta})}{f_X^{(0)}(\mathbf{x}_n | \boldsymbol{\theta}_\infty^{(0)}) f_Y^{(0)}(\mathbf{y}_n | \boldsymbol{\theta}_\infty^{(0)})} + \frac{1}{N} \sum_{n=1}^N \ln \frac{f_X^{(0)}(\mathbf{x}_n | \boldsymbol{\theta}_\infty^{(0)}) f_Y^{(0)}(\mathbf{y}_n | \boldsymbol{\theta}_\infty^{(0)})}{f_X^{(0)}(\mathbf{x}_n | \hat{\boldsymbol{\theta}}_N^{(0)}) f_Y^{(0)}(\mathbf{y}_n | \hat{\boldsymbol{\theta}}_N^{(0)})} \\ & - \frac{1}{N} \sum_{n=1}^N \ln \frac{f(\mathbf{x}_n, \mathbf{y}_n | \boldsymbol{\theta})}{f_{XY}^{(1)}(\mathbf{x}_n, \mathbf{y}_n | \boldsymbol{\theta}_\infty^{(1)})} - \frac{1}{N} \sum_{n=1}^N \ln \frac{f_{XY}^{(1)}(\mathbf{x}_n, \mathbf{y}_n | \boldsymbol{\theta}_\infty^{(1)})}{f_{XY}^{(1)}(\mathbf{x}_n, \mathbf{y}_n | \hat{\boldsymbol{\theta}}_N^{(1)})}. \end{aligned} \quad (\text{S-36})$$

According to the strong law of large numbers, the first and third sums in the right-hand side of the equation tend to

$$D_{\text{KL}} \left[ f(\mathbf{x}, \mathbf{y} | \boldsymbol{\theta}) \parallel f_X^{(0)}(\mathbf{x} | \boldsymbol{\theta}_\infty^{(0)}) f_Y^{(0)}(\mathbf{y} | \boldsymbol{\theta}_\infty^{(0)}) \right] \quad (\text{S-37})$$

and

$$D_{\text{KL}} \left[ f(\mathbf{x}, \mathbf{y} | \boldsymbol{\theta}) \parallel f_{XY}^{(1)}(\mathbf{x}, \mathbf{y} | \boldsymbol{\theta}_\infty^{(1)}) \right], \quad (\text{S-38})$$

respectively, while both the second and fourth sums tend to 0. Consequently, we obtain

$$J_N(D) = D_{\text{KL}} \left[ f(\mathbf{x}, \mathbf{y} | \boldsymbol{\theta}) \parallel f_X^{(0)}(\mathbf{x} | \boldsymbol{\theta}_\infty^{(0)}) f_Y^{(0)}(\mathbf{y} | \boldsymbol{\theta}_\infty^{(0)}) \right] - D_{\text{KL}} \left[ f(\mathbf{x}, \mathbf{y} | \boldsymbol{\theta}) \parallel f_{XY}^{(1)}(\mathbf{x}, \mathbf{y} | \boldsymbol{\theta}_\infty^{(1)}) \right] + o(1),$$

where  $o(\cdot)$  is the usual little-o notation, so that

$$\ln \frac{L_1(\hat{\boldsymbol{\theta}}_N^{(1)})}{L_0(\hat{\boldsymbol{\theta}}_N^{(0)})} = N \left\{ D_{\text{KL}} \left[ f(\mathbf{x}, \mathbf{y} | \boldsymbol{\theta}) \parallel f_X^{(0)}(\mathbf{x} | \boldsymbol{\theta}_\infty^{(0)}) f_Y^{(0)}(\mathbf{y} | \boldsymbol{\theta}_\infty^{(0)}) \right] - D_{\text{KL}} \left[ f(\mathbf{x}, \mathbf{y} | \boldsymbol{\theta}) \parallel f_{XY}^{(1)}(\mathbf{x}, \mathbf{y} | \boldsymbol{\theta}_\infty^{(1)}) \right] \right\} + o(N).$$

## 8 Bivariate normal distribution with noise

### 8.1 Graphical model

The graphical representation of the model can be found in Figure S-1.

### 8.2 Marginal model likelihood of $H_0$ .

The marginal model likelihood of  $H_0$  can be expressed as

$$p(D | H_0) = \int p(D | H_0, \mathbf{x}, \mathbf{y}) p(\mathbf{x}, \mathbf{y} | H_0) d\mathbf{x} d\mathbf{y}$$

with

$$p(\mathbf{x}, \mathbf{y} | H_0) = (2\pi\tau^2)^{-\frac{2N}{2}} \prod_{n=1}^N \exp \left( -\frac{x_n^2 + y_n^2}{2\tau^2} \right)$$

and

$$p(D | H_0, \mathbf{x}, \mathbf{y}) = (2\pi\sigma^2)^{-\frac{2N}{2}} \prod_{n=1}^N \exp \left\{ -\frac{1}{2\sigma^2} [(u_n - x_n)^2 + (v_n - y_n)^2] \right\},$$

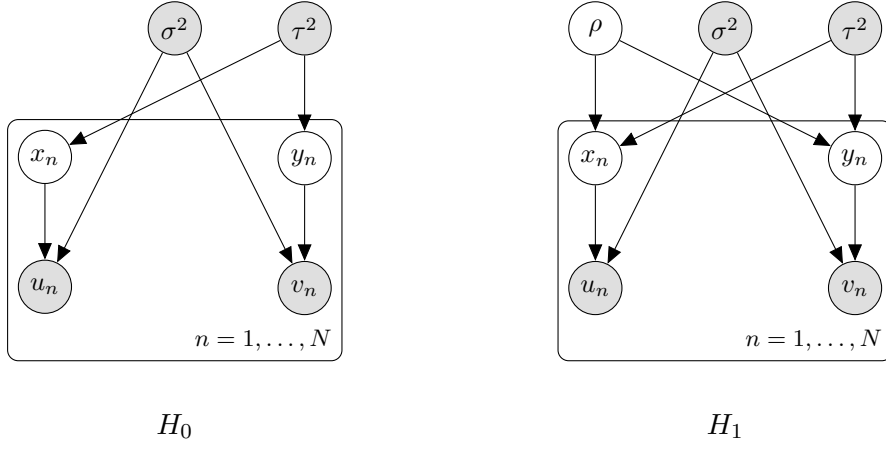

Figure S-1: **Simulation study: bivariate normal distribution with noise.** Bayesian networks coding the independence model  $H_0$  (left) and the dependence model  $H_1$  (right). Parameters whose values are known are represented in gray circles, and unknown parameters in white circles.

so that

$$\begin{aligned} p(D|H_0) &= (2\pi)^{-\frac{4N}{2}} (\sigma^2)^{-\frac{2N}{2}} (\tau^2)^{-\frac{2N}{2}} \prod_{n=1}^N \int \exp\left(-\frac{x_n^2 + y_n^2}{2\tau^2}\right) \\ &\quad \times \exp\left\{-\frac{1}{2\sigma^2} [(u_n - x_n)^2 + (v_n - y_n)^2]\right\} dx_n dy_n. \end{aligned}$$

Each quadratic term can be expanded as

$$\begin{aligned} \frac{(u_n - x_n)^2}{\sigma^2} + \frac{x_n^2}{\tau^2} &= \frac{u_n^2 + x_n^2 - 2u_n x_n}{\sigma^2} + \frac{x_n^2}{\tau^2} \\ &= \left(\frac{1}{\sigma^2} + \frac{1}{\tau^2}\right) x_n^2 - 2\frac{u_n}{\sigma^2} x_n + \frac{u_n^2}{\sigma^2} \\ &= \left(\frac{1}{\sigma^2} + \frac{1}{\tau^2}\right) (x_n - \hat{x}_n)^2 + \frac{u_n^2}{\sigma^2} - \left(\frac{1}{\sigma^2} + \frac{1}{\tau^2}\right) \hat{x}_n^2, \end{aligned}$$

with

$$\hat{x}_n = \frac{\frac{u_n}{\sigma^2}}{\frac{1}{\sigma^2} + \frac{1}{\tau^2}}$$

and

$$\begin{aligned} \frac{u_n^2}{\sigma^2} - \left(\frac{1}{\sigma^2} + \frac{1}{\tau^2}\right) \hat{x}_n^2 &= \frac{u_n^2}{\sigma^2} - \frac{\frac{u_n^2}{\sigma^4}}{\frac{1}{\sigma^2} + \frac{1}{\tau^2}} \\ &= \frac{u_n^2}{\sigma^2 + \tau^2}, \end{aligned}$$

so that

$$\frac{(u_n - x_n)^2}{\sigma^2} + \frac{x_n^2}{\tau^2} = \frac{\sigma^2 + \tau^2}{\sigma^2 \tau^2} (x_n - \hat{x}_n)^2 + \frac{u_n^2}{\sigma^2 + \tau^2}.$$

This leads to the following integration:

$$\int \exp\left\{-\frac{1}{2} \left[\frac{(u_n - x_n)^2}{\sigma^2} + \frac{x_n^2}{\tau^2}\right]\right\} dx_n = \exp\left[-\frac{u_n^2}{2(\sigma^2 + \tau^2)}\right] \sqrt{2\pi \left(\frac{\sigma^2 \tau^2}{\sigma^2 + \tau^2}\right)}.$$

Similarly,

$$\int \exp\left\{-\frac{1}{2} \left[\frac{(v_n - y_n)^2}{\sigma^2} + \frac{y_n^2}{\tau^2}\right]\right\} dy_n = \exp\left[-\frac{v_n^2}{2(\sigma^2 + \tau^2)}\right] \sqrt{2\pi \left(\frac{\sigma^2 \tau^2}{\sigma^2 + \tau^2}\right)}.$$

The marginal model likelihood then yields

$$p(D|H_0) = (2\pi)^{-\frac{2N}{2}} (\sigma^2 + \tau^2)^{-\frac{2N}{2}} \exp \left[ -\frac{\sum_{n=1}^N (u_n^2 + v_n^2)}{2(\sigma^2 + \tau^2)} \right].$$

### 8.3 Marginal model likelihood of $H_1$ .

Setting  $\mathbf{w}_n = (u_n, v_n)^\mathbf{t}$  and  $\mathbf{z}_n = (x_n, y_n)^\mathbf{t}$ , we obtain

$$p(D|H_1) = \int p(D|H_1, \mathbf{z}, \rho) p(\mathbf{z}|H_1, \rho) p(\rho|H_1) d\mathbf{z} d\rho,$$

with

$$p(\mathbf{z}|H_1, \rho) = (2\pi\tau^2)^{-\frac{2N}{2}} |\mathbf{M}(\rho)|^{-\frac{N}{2}} \prod_{n=1}^N \exp \left[ -\frac{1}{2\tau^2} \mathbf{z}_n^\mathbf{t} \mathbf{M}(\rho)^{-1} \mathbf{z}_n \right]$$

and

$$p(D|H_1, \mathbf{z}, \rho) = (2\pi\sigma^2)^{-\frac{2N}{2}} \prod_{n=1}^N \exp \left[ -\frac{1}{2\sigma^2} (\mathbf{w}_n - \mathbf{z}_n)^\mathbf{t} (\mathbf{w}_n - \mathbf{z}_n) \right],$$

so that

$$\begin{aligned} p(D|H_1) &= (2\pi)^{-\frac{4N}{2}} (\sigma^2)^{-\frac{2N}{2}} (\tau^2)^{-\frac{2N}{2}} \prod_{n=1}^N \int |\mathbf{M}(\rho)|^{-\frac{N}{2}} \exp \left[ -\frac{1}{2\tau^2} \mathbf{z}_n^\mathbf{t} \mathbf{M}(\rho)^{-1} \mathbf{z}_n \right] \\ &\quad \times \exp \left[ -\frac{1}{2\sigma^2} (\mathbf{w}_n - \mathbf{z}_n)^\mathbf{t} (\mathbf{w}_n - \mathbf{z}_n) \right] p(\rho|H_1) d\mathbf{z}_n d\rho. \end{aligned}$$

The quadratic terms can be expanded as

$$\begin{aligned} &\frac{1}{\sigma^2} (\mathbf{w}_n - \mathbf{z}_n)^\mathbf{t} (\mathbf{w}_n - \mathbf{z}_n) + \frac{1}{\tau^2} \mathbf{z}_n^\mathbf{t} \mathbf{M}(\rho)^{-1} \mathbf{z}_n \\ &= \mathbf{z}_n^\mathbf{t} \left[ \frac{1}{\sigma^2} \mathbf{I} + \frac{1}{\tau^2} \mathbf{M}(\rho)^{-1} \right] \mathbf{z}_n - \frac{2}{\sigma^2} \mathbf{z}_n^\mathbf{t} \mathbf{w}_n + \frac{1}{\sigma^2} \mathbf{w}_n^\mathbf{t} \mathbf{w}_n \\ &= (\mathbf{z}_n - \hat{\mathbf{z}}_n)^\mathbf{t} \left[ \frac{1}{\sigma^2} \mathbf{I} + \frac{1}{\tau^2} \mathbf{M}(\rho)^{-1} \right] (\mathbf{z}_n - \hat{\mathbf{z}}_n) + \frac{1}{\sigma^2} \mathbf{w}_n^\mathbf{t} \mathbf{w}_n - \hat{\mathbf{z}}_n^\mathbf{t} \left[ \frac{1}{\sigma^2} \mathbf{I} + \frac{1}{\tau^2} \mathbf{M}(\rho)^{-1} \right] \hat{\mathbf{z}}_n, \end{aligned}$$

with

$$\hat{\mathbf{z}}_n = \left[ \frac{1}{\sigma^2} \mathbf{I} + \frac{1}{\tau^2} \mathbf{M}(\rho)^{-1} \right]^{-1} \frac{1}{\sigma^2} \mathbf{w}_n$$

and

$$\begin{aligned} &\frac{1}{\sigma^2} \mathbf{w}_n^\mathbf{t} \mathbf{w}_n - \hat{\mathbf{z}}_n^\mathbf{t} \left[ \frac{1}{\sigma^2} \mathbf{I} + \frac{1}{\tau^2} \mathbf{M}(\rho)^{-1} \right] \hat{\mathbf{z}}_n \\ &= \frac{1}{\sigma^2} \left\{ \mathbf{w}_n^\mathbf{t} \mathbf{w}_n - \frac{1}{\sigma^2} \mathbf{w}_n^\mathbf{t} \left[ \frac{1}{\sigma^2} \mathbf{I} + \frac{1}{\tau^2} \mathbf{M}(\rho)^{-1} \right]^{-1} \mathbf{w}_n \right\} \\ &= \frac{1}{\sigma^2} \mathbf{w}_n^\mathbf{t} \left\{ \mathbf{I} - \left[ \mathbf{I} + \frac{\sigma^2}{\tau^2} \mathbf{M}(\rho)^{-1} \right]^{-1} \right\} \mathbf{w}_n \end{aligned}$$

so that

$$\begin{aligned} &\frac{1}{\sigma^2} (\mathbf{w}_n - \mathbf{z}_n)^\mathbf{t} (\mathbf{w}_n - \mathbf{z}_n) + \frac{1}{\tau^2} \mathbf{z}_n^\mathbf{t} \mathbf{M}(\rho)^{-1} \mathbf{z}_n \\ &= (\mathbf{z}_n - \hat{\mathbf{z}}_n)^\mathbf{t} \left[ \frac{1}{\sigma^2} \mathbf{I} + \frac{1}{\tau^2} \mathbf{M}(\rho)^{-1} \right] (\mathbf{z}_n - \hat{\mathbf{z}}_n) + \frac{1}{\sigma^2} \mathbf{w}_n^\mathbf{t} \left\{ \mathbf{I} - \left[ \mathbf{I} + \frac{\sigma^2}{\tau^2} \mathbf{M}(\rho)^{-1} \right]^{-1} \right\} \mathbf{w}_n. \end{aligned}$$

We then obtain the following integration

$$\begin{aligned} & \int \exp \left[ -\frac{1}{2\sigma^2} (\mathbf{w}_n - \mathbf{z}_n)^t (\mathbf{w}_n - \mathbf{z}_n) - \frac{1}{2\tau^2} \mathbf{z}_n^t \mathbf{M}(\rho)^{-1} \mathbf{z}_n \right] d\mathbf{z}_n \\ &= (2\pi) \left| \frac{1}{\sigma^2} \mathbf{I} + \frac{1}{\tau^2} \mathbf{M}(\rho)^{-1} \right|^{-\frac{1}{2}} \exp \left( -\frac{1}{2\sigma^2} \mathbf{w}_n^t \left\{ \mathbf{I} - \left[ \mathbf{I} + \frac{\sigma^2}{\tau^2} \mathbf{M}(\rho)^{-1} \right]^{-1} \right\} \mathbf{w}_n \right). \end{aligned}$$

The marginal model likelihood then yields

$$\begin{aligned} p(D|H_1) &= (2\pi)^{-\frac{2N}{2}} \int |\sigma^2 \mathbf{I} + \tau^2 \mathbf{M}(\rho)|^{-\frac{N}{2}} \\ &\quad \times \exp \left( -\frac{1}{2\sigma^2} \sum_{n=1}^N \mathbf{w}_n^t \left\{ \mathbf{I} - \left[ \mathbf{I} + \frac{\sigma^2}{\tau^2} \mathbf{M}(\rho)^{-1} \right]^{-1} \right\} \mathbf{w}_n \right) p(\rho|H_1) d\rho. \end{aligned}$$

Defining the sample sum-of-square matrix as

$$\mathbf{S} = \sum_{n=1}^N \mathbf{w}_n^t \mathbf{w}_n,$$

we are led to

$$\begin{aligned} p(D|H_1) &= (2\pi)^{-\frac{2N}{2}} \int |\sigma^2 \mathbf{I} + \tau^2 \mathbf{M}(\rho)|^{-\frac{N}{2}} \\ &\quad \times \exp \left[ -\frac{1}{2\sigma^2} \text{tr} \left( \mathbf{S} \left\{ \mathbf{I} - \left[ \mathbf{I} + \frac{\sigma^2}{\tau^2} \mathbf{M}(\rho)^{-1} \right]^{-1} \right\} \right) \right] p(\rho|H_1) d\rho. \end{aligned}$$

## 9 Functional dependence plus noise

### 9.1 Graphical model

The graphical representation of the model can be found in Figure S-2.

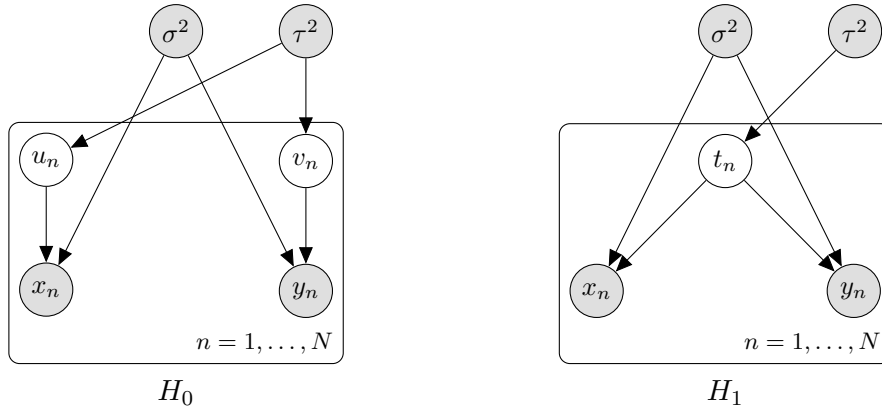

Figure S-2: **Simulation study: functional dependence plus noise.** Bayesian networks coding the independence model  $H_0$  (left) and the dependence model  $H_1$  (right). Parameters whose values are known are represented in gray circles, and unknown parameters in white circles.

### 9.2 Marginal model likelihood of $H_0$ .

The marginal model likelihood of  $H_0$  can be expressed as

$$p(D|H_0) = \int p(D|H_0, \mathbf{u}, \mathbf{v}) p(\mathbf{u}, \mathbf{v}|H_0) d\mathbf{u} d\mathbf{v}.$$

In this expression, we assume prior independence of the  $u_n$ 's and the  $v_n$ 's, so that

$$p(\mathbf{u}, \mathbf{v} | H_0) = \prod_{n=1}^N p(u_n | H_0) \prod_{n=1}^N p(v_n | H_0)$$

with

$$\begin{aligned} p(u_n | H_0) &= \mathcal{N}(u_n; 0, \tau^2) \\ &= \frac{1}{\sqrt{2\pi\tau^2}} \exp\left(-\frac{u_n^2}{2\tau^2}\right) \\ p(v_n | H_0) &= \mathcal{N}(v_n; 0, \tau^2) \\ &= \frac{1}{\sqrt{2\pi\tau^2}} \exp\left(-\frac{v_n^2}{2\tau^2}\right). \end{aligned}$$

As to the likelihood, it reads

$$p(D | H_0, \mathbf{u}, \mathbf{v}) = (2\pi\sigma^2)^{-\frac{2N}{2}} \prod_{n=1}^N \exp\left[-\frac{(x_n - u_n)^2}{2\sigma^2}\right] \prod_{n=1}^N \exp\left[-\frac{(y_n - v_n)^2}{2\sigma^2}\right],$$

so that

$$\begin{aligned} p(D | H_0) &= (2\pi)^{-\frac{4N}{2}} (\sigma^2)^{-\frac{2N}{2}} (\tau^2)^{-\frac{2N}{2}} \prod_{n=1}^N \int du_n \exp\left[-\frac{u_n^2}{2\tau^2} - \frac{(x_n - u_n)^2}{2\sigma^2}\right] \\ &\quad \times \prod_{n=1}^N \int dv_n \exp\left[-\frac{v_n^2}{2\tau^2} - \frac{(y_n - v_n)^2}{2\sigma^2}\right]. \end{aligned}$$

Each quadratic term in the exponential of the integrand in  $u_n$  can be expanded as

$$\begin{aligned} \frac{(x_n - u_n)^2}{\sigma^2} + \frac{u_n^2}{\tau^2} &= \frac{x_n^2 + u_n^2 - 2x_n u_n}{\sigma^2} + \frac{u_n^2}{\tau^2} \\ &= \left(\frac{1}{\sigma^2} + \frac{1}{\tau^2}\right) u_n^2 - 2\frac{x_n}{\sigma^2} u_n + \frac{x_n^2}{\sigma^2} \\ &= \left(\frac{1}{\sigma^2} + \frac{1}{\tau^2}\right) (u_n - \hat{u}_n)^2 + \frac{x_n^2}{\sigma^2} - \left(\frac{1}{\sigma^2} + \frac{1}{\tau^2}\right) \hat{u}_n^2, \end{aligned}$$

with

$$\hat{u}_n = \frac{\frac{x_n}{\sigma^2}}{\frac{1}{\sigma^2} + \frac{1}{\tau^2}}$$

and

$$\begin{aligned} \frac{x_n^2}{\sigma^2} - \left(\frac{1}{\sigma^2} + \frac{1}{\tau^2}\right) \hat{u}_n^2 &= \frac{x_n^2}{\sigma^2} - \frac{\frac{x_n^2}{\sigma^4}}{\frac{1}{\sigma^2} + \frac{1}{\tau^2}} \\ &= \frac{x_n^2}{\sigma^2 + \tau^2}, \end{aligned}$$

so that

$$\frac{(x_n - u_n)^2}{\sigma^2} + \frac{u_n^2}{\tau^2} = \frac{\sigma^2 + \tau^2}{\sigma^2 \tau^2} (u_n - \hat{u}_n)^2 + \frac{x_n^2}{\sigma^2 + \tau^2}.$$

This leads to the following integration:

$$\int \exp\left\{-\frac{1}{2} \left[\frac{(x_n - u_n)^2}{\sigma^2} + \frac{u_n^2}{\tau^2}\right]\right\} du_n = \exp\left[-\frac{x_n^2}{2(\sigma^2 + \tau^2)}\right] \sqrt{2\pi \left(\frac{\sigma^2 \tau^2}{\sigma^2 + \tau^2}\right)}.$$

Similarly,

$$\int \exp \left\{ -\frac{1}{2} \left[ \frac{(y_n - v_n)^2}{\sigma^2} + \frac{v_n^2}{\tau^2} \right] \right\} dv_n = \exp \left[ -\frac{y_n^2}{2(\sigma^2 + \tau^2)} \right] \sqrt{2\pi \left( \frac{\sigma^2 \tau^2}{\sigma^2 + \tau^2} \right)}.$$

The marginal model likelihood then yields

$$p(D|H_0) = (2\pi)^{-\frac{2N}{2}} (\sigma^2 + \tau^2)^{-\frac{2N}{2}} \exp \left[ -\frac{\sum_{n=1}^N (x_n^2 + y_n^2)}{2(\sigma^2 + \tau^2)} \right].$$

and the log

$$\ln p(D|H_0) = -\frac{2N}{2} \ln(2\pi) - \frac{2N}{2} \ln(\sigma^2 + \tau^2) - \sum_{n=1}^N \frac{x_n^2 + y_n^2}{2(\sigma^2 + \tau^2)}.$$

### 9.3 Marginal model likelihood of $H_1$ .

The marginal model likelihood of  $H_0$  can be expressed as

$$p(D|H_1) = \int p(D|H_0, \mathbf{t}) p(\mathbf{t}|H_0) d\mathbf{t}$$

with

$$p(\mathbf{t}|H_1) = (2\pi\tau^2)^{-\frac{N}{2}} \prod_{n=1}^N \exp \left( -\frac{t_n^2}{2\tau^2} \right)$$

and

$$p(D|H_1, \mathbf{t}) = (2\pi\sigma^2)^{-\frac{2N}{2}} \prod_{n=1}^N \exp \left\{ -\frac{1}{2\sigma^2} [(x_n - t_n)^2 + (y_n - t_n)^2] \right\},$$

so that

$$\begin{aligned} p(D|H_1) &= (2\pi)^{-\frac{3N}{2}} (\sigma^2)^{-\frac{2N}{2}} (\tau^2)^{-\frac{N}{2}} \prod_{n=1}^N \int \exp \left( -\frac{t_n^2}{2\tau^2} \right) \\ &\quad \times \exp \left\{ -\frac{1}{2\sigma^2} [(x_n - t_n)^2 + (y_n - t_n)^2] \right\} dt_n. \end{aligned}$$

Each quadratic term can be expanded as

$$\begin{aligned} \frac{(x_n - t_n)^2}{\sigma^2} + \frac{(y_n - t_n)^2}{\sigma^2} + \frac{t_n^2}{\tau^2} &= \frac{2t_n^2 + x_n^2 + y_n^2 - 2t_n(x_n + y_n)}{\sigma^2} + \frac{t_n^2}{\tau^2} \\ &= \left( \frac{2}{\sigma^2} + \frac{1}{\tau^2} \right) t_n^2 - 2\frac{x_n + y_n}{\sigma^2} t_n + \frac{x_n^2 + y_n^2}{\sigma^2} \\ &= \left( \frac{2}{\sigma^2} + \frac{1}{\tau^2} \right) (t_n - \hat{t}_n)^2 + \frac{x_n^2 + y_n^2}{\sigma^2} - \left( \frac{2}{\sigma^2} + \frac{1}{\tau^2} \right) \hat{t}_n^2, \end{aligned}$$

with

$$\hat{t}_n = \frac{\frac{x_n + y_n}{\sigma^2}}{\frac{2}{\sigma^2} + \frac{1}{\tau^2}}$$

and

$$\begin{aligned} \frac{x_n^2 + y_n^2}{\sigma^2} - \left( \frac{2}{\sigma^2} + \frac{1}{\tau^2} \right) \hat{t}_n^2 &= \frac{x_n^2 + y_n^2}{\sigma^2} - \frac{\frac{x_n^2 + y_n^2 + 2x_n y_n}{\sigma^4}}{\frac{2}{\sigma^2} + \frac{1}{\tau^2}} \\ &= \frac{1}{\sigma^2} \frac{1}{2 + \frac{\sigma^2}{\tau^2}} \left[ \left( 2 + \frac{\sigma^2}{\tau^2} \right) (x_n^2 + y_n^2) - x_n^2 - y_n^2 - 2x_n y_n \right] \\ &= \frac{1}{\sigma^2} \frac{1}{2 + \frac{\sigma^2}{\tau^2}} \left[ (x_n - y_n)^2 + \frac{\sigma^2}{\tau^2} (x_n^2 + y_n^2) \right] \\ &= \frac{(x_n - y_n)^2}{\sigma^2(2 + \alpha^2)} + \frac{x_n^2 + y_n^2}{\tau^2(2 + \alpha^2)}, \end{aligned}$$

where we set  $\alpha^2 = \sigma^2/\tau^2$ . This leads us to

$$\frac{(x_n - t_n)^2 + (y_n - t_n)^2}{\sigma^2} + \frac{t_n^2}{\tau^2} = \frac{\sigma^2 + 2\tau^2}{\sigma^2\tau^2}(t_n - \hat{t}_n)^2 + \frac{(x_n - y_n)^2}{\sigma^2(2 + \alpha^2)} + \frac{x_n^2 + y_n^2}{\tau^2(2 + \alpha^2)}.$$

This leads to the following integration:

$$\begin{aligned} & \int \exp \left\{ -\frac{1}{2} \left[ \frac{(x_n - t_n)^2 + (y_n - t_n)^2}{\sigma^2} + \frac{t_n^2}{\tau^2} \right] \right\} dt_n \\ &= \exp \left[ -\frac{(x_n - y_n)^2}{2\sigma^2(2 + \alpha^2)} - \frac{x_n^2 + y_n^2}{2\tau^2(2 + \alpha^2)} \right] \sqrt{2\pi \left( \frac{\sigma^2\tau^2}{\sigma^2 + 2\tau^2} \right)}. \end{aligned}$$

The marginal model likelihood then yields

$$p(D|H_1) = (2\pi)^{-\frac{2N}{2}} (\sigma^2)^{-\frac{N}{2}} (\sigma^2 + 2\tau^2)^{-\frac{N}{2}} \prod_{n=1}^N \exp \left[ -\frac{(x_n - y_n)^2}{2\sigma^2(2 + \alpha^2)} - \frac{x_n^2 + y_n^2}{2\tau^2(2 + \alpha^2)} \right]$$

and the log

$$\begin{aligned} \ln p(D|H_1) &= -\frac{2N}{2} \ln(2\pi) - \frac{N}{2} \ln(\sigma^2) - \frac{N}{2} \ln(\sigma^2 + 2\tau^2) \\ &\quad - \sum_{n=1}^N \left[ \frac{(x_n - y_n)^2}{2\sigma^2(2 + \alpha^2)} + \frac{x_n^2 + y_n^2}{2\tau^2(2 + \alpha^2)} \right] \end{aligned}$$

## 10 Phase synchronization of chaotic systems

The system is composed of two coupled oscillators. Each oscillator  $i \in \{1, 2\}$  is characterized by its position  $(x_i, y_i, z_i)$  and its time derivatives  $(\dot{x}_i, \dot{y}_i, \dot{z}_i)$ . Their dynamics respects the following differential equation

$$\begin{cases} \dot{x}_i &= -\omega_i y_i - z_i + C(x_j - x_i) \\ \dot{y}_i &= \omega_i x_i + a y_i \\ \dot{z}_i &= f + z_i(x_i - c) \end{cases} \quad i \in \{1, 2\}, j \in \{1, 2\} \setminus \{i\}. \quad (\text{S-39})$$

We set  $a = 0.165$ ,  $f = 0.2$ ,  $c = 10$  (same values for both oscillators);  $\omega_1 = \omega_0 - \Delta\omega$  and  $\omega_2 = \omega_0 + \Delta\omega$ , with  $\omega_0 = 0.97$  and  $\Delta\omega = 0.02$ .  $C$  is the coupling parameter ( $C = 0$  corresponds to no coupling). We simulated data with  $C \in \{0, 10^{-3}, 10^{-2}, 0.1, 1\}$ . For a given set of parameter values, the trajectory of the system was generated numerically with an explicit Runge-Kutta method and downsampled to 1 s. Gaussian white noise is then added with variance  $\sigma^2 \in \{10^{-3}, 10^{-2}, 0.1, 1\}$ .

For the inference, the parameters were optimized by numerical maximization of the log-likelihood function (simplex search, Lagarias et al., 1998). Values of  $\mathfrak{B}_{\ln}(\mathcal{X}, \mathcal{Y}|D)$  were then computed using the BIC approximation.

## 11 Real-life application

### 11.1 Case of independence

Under  $H_0$ , we have

$$p(\theta_n) = \frac{1}{2\pi},$$

so that the likelihood reads

$$p(D|H_0) = \left( \frac{1}{2\pi} \right)^N.$$

## 11.2 Case of dependence

By contrast, under  $H_1$ , the likelihood reads (Mardia and Jupp, 2000, §3.5.4)

$$p(\theta_n|H_1, \mu, \kappa) = \frac{1}{2\pi I_0(\kappa)} \exp[\kappa \cos(\theta_n - \mu)],$$

where  $I_0(\kappa)$  is the modified Bessel function of the first kind and order 0,

$$I_0(\kappa) = \frac{1}{2\pi} \int_0^{2\pi} \exp[\kappa \cos(\theta)] d\theta.$$

The likelihood can be rearranged to yield (Marrelec and Giron, 2024)

$$p(D|H_1, \mu, \kappa) = \left[ \frac{1}{2\pi I_0(\kappa)} \right]^N \exp[\kappa N \bar{R} \cos(\mu - m)],$$

where  $\bar{R}e^{im}$  is the sample circular mean of the data. The prior for  $\mu$  can be set as a noninformative, uniform prior over the circle,

$$p(\mu|H_1) = \frac{1}{2\pi}.$$

For  $\kappa$ , we use (Dowe et al., 1996)

$$p(\kappa|H_1) = \frac{\kappa}{(1 + \kappa^2)^{\frac{3}{2}}}, \quad \kappa \geq 0.$$

$p(D|H_1)$  can then be expressed as

$$p(D|H_1) = (2\pi)^{-(N+1)} \int \frac{\kappa}{(1 + \kappa^2)^{\frac{3}{2}}} I_0(\kappa)^{-N} \exp[\kappa N \bar{R} \cos(\mu - m)] d\mu d\kappa.$$

Integration with respect to  $\mu$  can be performed in closed form, yielding

$$p(D|H_1) = (2\pi)^{-N} \int \frac{\kappa}{(1 + \kappa^2)^{\frac{3}{2}}} \frac{I_0(N\bar{R}\kappa)}{I_0(\kappa)^N} d\kappa.$$

## 11.3 Measure of dependence

Finally,  $\mathfrak{B}_{\text{ln}}(\mathcal{X}, \mathcal{Y}|D)$  reads

$$\mathfrak{B}_{\text{ln}}(\mathcal{X}, \mathcal{Y}|D) = \ln \frac{p(H_1)}{p(H_0)} + \ln \left[ \int \frac{\kappa}{(1 + \kappa^2)^{\frac{3}{2}}} \frac{I_0(N\bar{R}\kappa)}{I_0(\kappa)^N} d\kappa \right].$$

# 12 The case of the log Bayes ratio per sample

## 12.1 Definition

We define the log Bayes ratio per sample as

$$\mathfrak{N}(\mathcal{X}, \mathcal{Y}|D) \equiv \frac{1}{N} \mathfrak{B}_{\text{lnr}}(\mathcal{X}, \mathcal{Y}|D) = \frac{1}{N} \ln \frac{p(H_1|D)}{p(H_0|D)},$$

which quantifies the log increase in favor of  $H_1$  per sample. Its theoretical lower and upper bounds are  $-\infty$  and  $+\infty$ , respectively.

## 12.2 Calculations

In the calculations,  $\mathfrak{N}(\mathcal{X}, \mathcal{Y}|D)$  behaves very similarly to mutual information.

**Known distributions.** In the case of a known joint distribution of the form  $f_X^{(0)}(\mathbf{x}) f_Y^{(0)}(\mathbf{y})$  for  $H_0$  and  $f_{XY}^{(1)}(\mathbf{x}, \mathbf{y})$  for  $H_1$ , we obtain from Equation (S-1):

$$\mathfrak{N}(\mathcal{X}, \mathcal{Y}|D) = \frac{1}{N} \ln \frac{P(H_1)}{P(H_0)} + \frac{1}{N} \sum_{n=1}^N \ln \frac{f_{XY}^{(1)}(\mathbf{x}_n, \mathbf{y}_n)}{f_X^{(0)}(\mathbf{x}_n) f_Y^{(0)}(\mathbf{y}_n)}.$$

Since the  $(\mathbf{x}_n, \mathbf{y}_n)$ 's are independent for different values of  $n$ , so are the corresponding values of

$$\ln \frac{f_{XY}^{(1)}(\mathbf{x}_n, \mathbf{y}_n)}{f_X^{(0)}(\mathbf{x}_n) f_Y^{(0)}(\mathbf{y}_n)}.$$

One can thus apply the law of large numbers. Under  $H_0$ , it yields

$$\frac{1}{N} \sum_{n=1}^N \ln \frac{f_{XY}^{(1)}(\mathbf{x}_n, \mathbf{y}_n)}{f_X^{(0)}(\mathbf{x}_n) f_Y^{(0)}(\mathbf{y}_n)} \xrightarrow{N \rightarrow \infty} \int f_X^{(0)}(\mathbf{x}) f_Y^{(0)}(\mathbf{y}) \ln \frac{f_{XY}^{(1)}(\mathbf{x}, \mathbf{y})}{f_X^{(0)}(\mathbf{x}) f_Y^{(0)}(\mathbf{y})} d\mathbf{x} d\mathbf{y} = -D_{\text{KL}}(f_X^{(0)} f_Y^{(0)} \| f_{XY}^{(1)}),$$

leading to  $\mathfrak{N}(\mathcal{X}, \mathcal{Y}|D) \xrightarrow{N \rightarrow \infty} -D_{\text{KL}}(f_X^{(0)} f_Y^{(0)} \| f_{XY}^{(1)})$ . By contrast, under  $H_1$ , we are led to

$$\frac{1}{N} \sum_{n=1}^N \ln \frac{f_{XY}^{(1)}(\mathbf{x}_n, \mathbf{y}_n)}{f_X^{(0)}(\mathbf{x}_n) f_Y^{(0)}(\mathbf{y}_n)} \xrightarrow{N \rightarrow \infty} \int f_{XY}^{(1)}(\mathbf{x}, \mathbf{y}) \ln \frac{f_{XY}^{(1)}(\mathbf{x}, \mathbf{y})}{f_X^{(0)}(\mathbf{x}) f_Y^{(0)}(\mathbf{y})} d\mathbf{x} d\mathbf{y} = I(X, Y),$$

so that  $\mathfrak{N}(\mathcal{X}, \mathcal{Y}|D)$  tends to  $I(X, Y)$  as  $N \rightarrow \infty$ .

**Maximum-entropy distributions.** We obtain from Equation (S-19)

$$\mathfrak{N}(\mathcal{X}, \mathcal{Y}|D) = \hat{I}(X, Y) - \frac{(D_1 - D_0) \ln N}{2} + O\left(\frac{1}{N}\right) \xrightarrow{N \rightarrow \infty} I(X, Y). \quad (\text{S-40})$$

**Multivariate normal distributions.** Equation (S-21) leads us to

$$\mathfrak{N}(\mathcal{X}, \mathcal{Y}|D) = \hat{I}(X, Y) - \frac{D_X D_Y \ln N}{2} + O\left(\frac{1}{N}\right) \xrightarrow{N \rightarrow \infty} I(X, Y),$$

**Bivariate discrete distributions.** From Equation (S-33), we obtain

$$\mathfrak{N}(\mathcal{X}, \mathcal{Y}|D) = \hat{I}(X, Y) - \frac{(r-1)(s-1) \ln N}{2} + O\left(\frac{1}{N}\right) \xrightarrow{N \rightarrow \infty} I(X, Y).$$

### 12.3 Simulation studies

**Bivariate normal distribution with noise.** Results are summarized in Figure S-3.  $\mathfrak{N}(\mathcal{X}, \mathcal{Y}|D)$  tended to  $I(X, Y)$  with increasing  $N$  and decreasing  $\sigma^2$ . However, it was not a decreasing function of  $N$  towards its lower bound  $(-\infty)$  for  $H_0$ . For  $H_1$ , it did not tend to its upper bound  $(+\infty)$  as  $N \rightarrow \infty$ .

**Functional dependence with noise.** The results are summarized in Figure S-4.  $\mathfrak{N}(\mathcal{X}, \mathcal{Y}|D)$  was relatively constant with respect to  $N$ , with a sign that was negative for  $H_0$  and positive for  $H_1$ , and an absolute value that decreased with increasing  $\sigma^2$ . In particular, unlike other cases considered so far,  $\mathfrak{N}(\mathcal{X}, \mathcal{Y}|D)$  tended toward a negative value. Since that value was negative, it could not be associated with mutual information (which has to be non-negative).

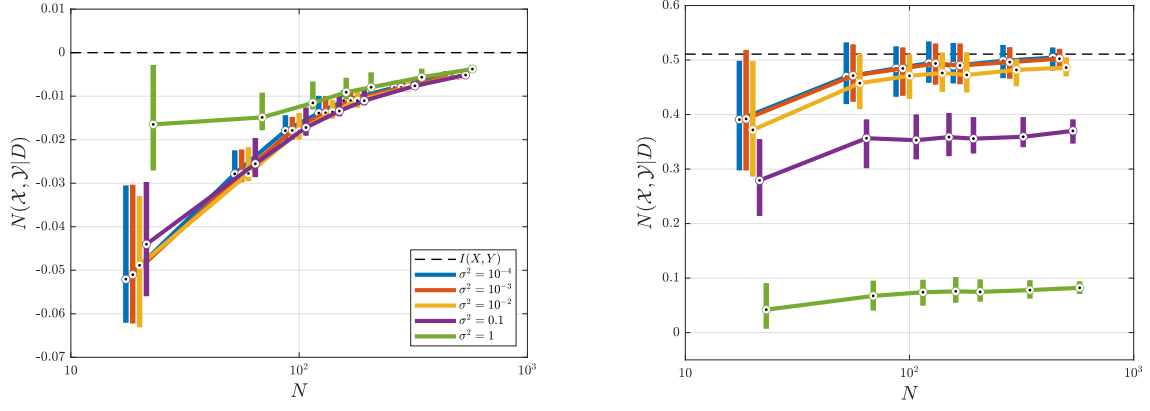

Figure S-3: **Simulation study: bivariate normal distribution with noise.** Boxplots (median and [25%, 75%] percentile interval) of  $\mathfrak{N}(\mathcal{X}, \mathcal{Y}|D)$  when  $H_0$  is true (left) or when  $H_1$  is true with  $\rho = 0.8$  (right).

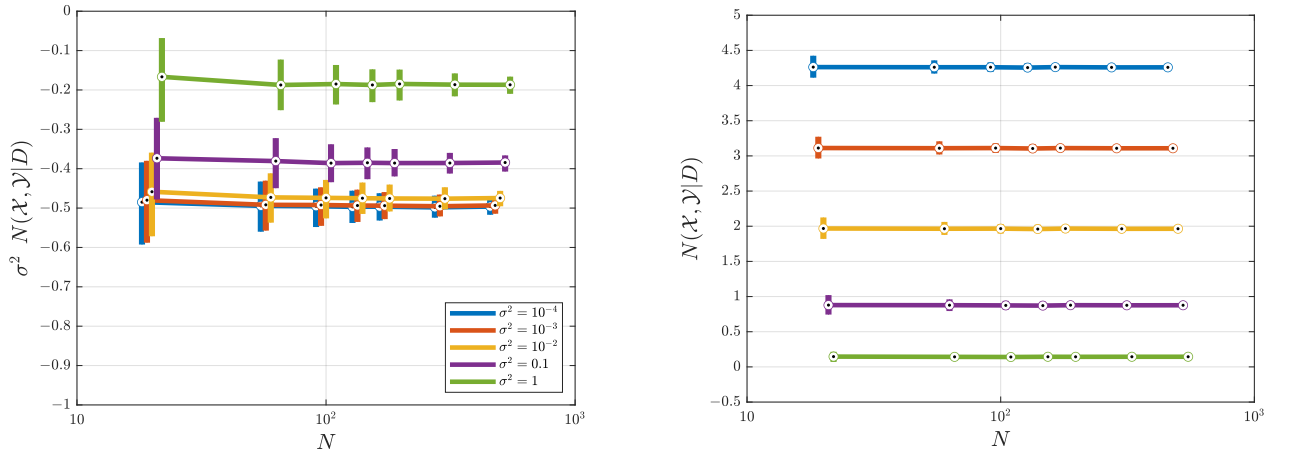

Figure S-4: **Simulation study: functional dependence with noise.** Boxplots of the effect of  $\sigma^2$  and  $N$  on  $\mathfrak{N}(\mathcal{X}, \mathcal{Y}|D)$  when  $H_0$  is true (left) or when  $H_1$  is true (right).

## 12.4 Summary

The various results (calculations and simulation study) emphasize the connection between  $\mathfrak{N}(\mathcal{X}, \mathcal{Y}|D)$  and mutual information, in that  $\mathfrak{N}(\mathcal{X}, \mathcal{Y}|D)$  often tends to  $I(X, Y)$  as  $N \rightarrow \infty$ . This shows that  $\mathfrak{N}(\mathcal{X}, \mathcal{Y}|D)$  is often a reasonable estimator of  $I(X, Y)$ . However, it also implies that

- In the case of no dependence (as modeled by  $H_0$ ),  $\mathfrak{N}(\mathcal{X}, \mathcal{Y}|D)$  tends to 0 (and not its lower bound,  $-\infty$ );
- In the case of a dependence (as modeled by  $H_1$ ), then  $\mathfrak{N}(\mathcal{X}, \mathcal{Y}|D)$  tends to a strictly positive value (and not its upper bound,  $+\infty$ ).

As a consequence, the range of values that  $\mathfrak{N}(\mathcal{X}, \mathcal{Y}|D)$  can reach is much more limited than its theoretical range of  $]-\infty, +\infty[$ . Also, it is not typically a monotonous (decreasing for  $H_0$ , increasing for  $H_1$ ) function of the quantity of information contained in the data.

## 13 Mutual information for the simulation study

In the case of the simulation study involving a bivariate normal distribution with noise (Section III-A of the manuscript), we expect  $\hat{I}(U, V)$ , the naive estimator for a bivariate normal distribution from Equation (S-22) applied to our data  $(u_n, v_n)$ , to be a good estimator of  $I(X, Y)$  only when  $\sigma^2 \ll \tau^2$  and  $N$  is large. When this assumption is not valid, an ad hoc estimator  $\tilde{I}(X, Y)$  of  $I(X, Y)$  could be proposed using the fact that  $\text{Cov}(U, V) = \text{Cov}(X, Y)$ , yielding

$$\tilde{I}(X, Y) = -\frac{1}{2} \ln(1 - \tilde{\rho}^2),$$

with

$$\tilde{\rho} = \frac{\widehat{\text{Cov}(U, V)}}{\tau^2}.$$

However, the theoretical and practical properties of this estimator, as well as its actual value in the case of the simulation study, remain unclear to the authors.

By contrast, in the case of the simulation study involving a functional dependence with noise, we are not even aware of how information-theoretic measures could provide a relevant measure of dependence.

## References

- Abramovich, F., Ritov, Y., 2013. Statistical Theory: A Concise Introduction. Texts in Statistical Science, Chapman & Hall / CRC.
- Abramowitz, M., Stegun, I.A. (Eds.), 1972. Handbook of Mathematical Functions. Number 55 in Applied Math., National Bureau of Standards.
- Anderson, T.W., 1958. An Introduction to Multivariate Statistical Analysis. Wiley Publications in Statistics, John Wiley and Sons, New York.
- Anderson, T.W., 2003. An Introduction to Multivariate Statistical Analysis. Wiley Series in Probability and Mathematical Statistics. 3rd ed., John Wiley and Sons, New York.
- Bernardo, J.M., Smith, A.F.M., 2000. Bayesian Theory. Wiley Series in Probability and Mathematical Statistics. 3rd ed., Wiley & Sons, Chicester.
- Cover, T.M., Thomas, J.A., 1991. Elements of Information Theory. Wiley Series in Telecommunications and Signal Processing, Wiley.

- Dowe, D.L., Oliver, J.J., Baxter, R.A., Wallace, C.S., 1996. Bayesian estimation of the von Mises concentration parameter, in: Hanson, K.M., Silver, R.N. (Eds.), *Maximum Entropy and Bayesian Methods. Fundamental Theories of Physics*, Springer, Dordrecht. pp. 51–60.
- Gelfand, A.E., Dey, D.K., 1994. Bayesian model choice: Asymptotics and exact calculations. *Journal of the Royal Statistical Society: Series B (Statistical Methodology)* 56, 501–514.
- Gelman, A., Carlin, J.B., Stern, H.S., Rubin, D.B., 2004. *Bayesian Data Analysis. Texts in Statistical Science*. 2nd ed., Chapman & Hall, London.
- Jaynes, E.T., 2003. *Probability Theory: The Logic of Science*. Cambridge University Press, Cambridge.
- Kullback, S., 1968. *Information Theory and Statistics*. Dover, Mineola, NY.
- Lagarias, J.C., Reeds, J.A., Wright, M.H., Wright, P.E., 1998. Convergence properties of the Nelder–Mead simplex method in low dimensions. *SIAM Journal on Optimization* 9, 112–147.
- Mardia, K.V., Jupp, P.E., 2000. *Directional Statistics. Wiley Series in Probability and Statistics*, Wiley, Chichester.
- Marrelec, G., Giron, A., 2021. Automated extraction of mutual independence patterns using bayesian comparison of partition models. *IEEE Transactions on Pattern Analysis and Machine Intelligence* 43, 2299–2313.
- Marrelec, G., Giron, A., 2024. Estimating the concentration parameter of a von Mises distribution: a systematic simulation benchmark. *Communications in Statistics – Simulation and Computation* 53, 117–129.
- Marrelec, G., Messé, A., Bellec, P., 2015. A Bayesian alternative to mutual information for the hierarchical clustering of dependent random variables. *PLoS ONE* 10, e0137278.
- O’Hagan, A., Forster, J., 2004. *Kendall’s Advanced Theory of Statistics: Vol. 2B: Bayesian Inference*. Arnold, London.
- Press, S.J., 2005. *Applied Multivariate Analysis. Using Bayesian and Frequentist Methods of Inference*. 2nd ed., Dover, Mineola.
- Schwarz, G., 1978. Estimating the dimension of a model. *The Annals of Statistics* 6, 461–464.
- Tierney, L., Kadane, J.B., 1986. Accurate approximations for posterior moments and marginal densities. *Journal of the American Statistical Association* 81, 82–86.
- Whittaker, J., 1990. *Graphical Models in Applied Multivariate Statistics. J. Wiley and Sons*, Chichester.
- Wolf, D.R., 1994. Mutual information as a Bayesian measure of independence. *arXiv:comp-gas/9511002*.
